# Supplementary material for: Model selection in extreme value regression for estimation of changes in return values over time applied to extreme annual regional CMIP6 desert temperatures
Source: arXiv:2603.07227 source file (2026-08-25)
Supplement: Supplementary file 1 [file LchEA-ClimateCoupledTemperatures-SM.tex]

\documentclass{article}

\usepackage{amsmath}
\usepackage{amssymb}
\usepackage{xcolor}
\usepackage{xspace}
\usepackage{placeins}
\usepackage{graphicx}
\usepackage{caption}
\usepackage{pgffor}

\newif\ifNms
%\Nmstrue % Sets the condition to true
\Nmsfalse % Sets the condition to false

\ifNms
	\usepackage[round, authoryear]{natbib}
\else
	\usepackage[numbers]{natbib}
	\renewcommand{\citealt}{\cite}
\fi

\usepackage{subcaption} %for subfigure
\usepackage{url}

\oddsidemargin  -0.5in
\evensidemargin -0.5in
\textwidth      7.5in
\headheight     0.0in
\topmargin      -1.0in
\textheight     10.0in

\providecommand{\TA}{\texttt{tas}\xspace}

\providecommand{\AC}{\texttt{ACCESS-CM2}\xspace}

\providecommand{\CE}{\texttt{CESM2}\xspace}
\providecommand{\EC}{\texttt{EC-Earth3}\xspace}
\providecommand{\MR}{\texttt{MRI-ESM2-0}\xspace}

\providecommand{\UK}{\texttt{UKESM1-0-LL}\xspace}

\providecommand{\SL}{\texttt{SSP126}\xspace}
\providecommand{\SM}{\texttt{SSP245}\xspace}
\providecommand{\SH}{\texttt{SSP585}\xspace}

\providecommand{\DAN}{{Antarctic}\xspace}
\providecommand{\DDA}{{Dasht-e Lut}\xspace}
\providecommand{\DMO}{{Mojave}\xspace}
\providecommand{\DSA}{{Sahara}\xspace}
\providecommand{\DSI}{{Simpson}\xspace}
\providecommand{\DUK}{{UK}\xspace}

\newcommand {\argmax}[1]{\underset{#1}{\mathrm{argmax} \text{ }}}

\setlength{\parindent}{0pt}
\setlength{\parskip}{1em}

\title{\textbf{Supplementary Material}\\$\quad$\\Estimating changes in extreme quantiles over time, applied to desert temperatures}
\author{Callum Leach, Kevin Ewans, Philip Jonathan}
\date{}

\begin{document}
	\maketitle
	
	\renewcommand{\thesection}{SM\arabic{section}} % Adds SM prefix to the figure number
	\renewcommand{\thefigure}{SM\arabic{figure}} % Adds SM prefix to the figure number
	\renewcommand{\thetable}{SM\arabic{table}} % Adds SM prefix to the figure number
	\renewcommand{\theequation}{SM\arabic{equation}} % Adds SM prefix to the figure number

	%%%%%%%%%%%%%%%%%%%%%%%%%%%%%%%%%%%%%%%%%%%%%%%%%%%%%%%%%%%%%%%%%%
	\section*{Overview} \label{Ovr}
	%%%%%%%%%%%%%%%%%%%%%%%%%%%%%%%%%%%%%%%%%%%%%%%%%%%%%%%%%%%%%%%%%%
	
	This supplementary material provides supporting information for the article referenced above. 
	
	Section~\ref{SM:Ltr} provides further discussion of the literature on information criteria (such as AIC, BIC, DIC and WAIC), and non-stationary parametric GEV regression, to complement Section~1.

	Section~\ref{SM:TS} provides illustrations of regional annual minima time series for comparison with Figure~3.

	Section~\ref{SM:MCMC} provides a brief outline of the MCMC scheme for model parameter estimation, discussed in Section~3.2.

	Section~\ref{SM:Mxm} provides visual summaries of model fits for regional annual maxima (to be compared with Figure~6), and box-whisker plots of differences in return values $\Delta Q$ (to be compared with Figures~7-8).

	Section~\ref{SM:Mnm} provides visual summaries of model fits for regional annual minima (to be compared with corresponding figures for regional annual maxima in Figure~6 and Section~\ref{SM:Mxm}), and box-whisker plots of differences in return values for regional annual minima (to be compared with Figures~7-8).

	Section~\ref{SM:MxmMnmDff} gives box-whisker plots of $\Delta Q(\text{for maxima}) - \Delta Q(\text{for minima})$, comparing $\Delta Q$ for regional annual maxima and minima.

	Section~\ref{SM:LctMxmMnm} investigates the spatial distribution of regional annual maxima and minima

	Section~\ref{SM:DstMdlCmp} illustrates the distribution of complexity of fitted models (to be compared with Figure~11)

	Section~\ref{SM:BMA} provides some background to the Bayesian model averaging performed in Section~6.3.

	%%%%%%%%%%%%%%%%%%%%%%%%%%%%%%%%%%%%%%%%%%%%%%%%%%%%%%%%%%%%%%%%%%
	\clearpage
	\FloatBarrier
	\section{Literature review} \label{SM:Ltr}
	%%%%%%%%%%%%%%%%%%%%%%%%%%%%%%%%%%%%%%%%%%%%%%%%%%%%%%%%%%%%%%%%%%
	%
	This section should be read in conjunction with Section~1 of the main text.
	
	\subsection{Motivating the application} \label{SM:Ltr:App}
	Our planet's climate is changing due to human activity. Projections under specified future emissions scenarios using global climate models (GCMs) allow assessment of risk to society, and the efficacy of remedial actions. Large uncertainties in projections remain, especially at local scales (see e.g. \citealt{SmpEA25}). Some of the greatest societal impacts are caused by changes in mean characteristics of variables quantifying the state of the Earth's atmosphere and oceans. The fidelity with which these changes are encoded in GCMs can be assessed by comparing climate model output with observation. Other important impacts are caused by extremes, including heatwaves and storms. It is therefore critical also to understand the characteristics of projections of extremes from GCMs. Near-surface atmospheric temperature (\TA) is a critical output of global climate models; it is widely observed, it is the variable most commonly used to define global warming. It is typically projected to increase under all emission scenarios, and it is a key parameter in physical processes. In particular, the Sixth Assessment Report of the Intergovernmental Panel on Climate Change (\citealt{IPCC-2023SPM}) concludes with high to very high confidence that continued increases in global \TA will lead to systematic intensification of climate impacts, with severities strongly dependent on the magnitude of warming. For example, it is virtually certain that the frequency and intensity of hot extremes, including heatwaves, will increase as global mean near-surface temperature rises.
	
	\subsection{Information criteria} \label{SM:Ltr:ICs}
	\cite{ZhnEA23} gives a more recent review of the use of information criteria for statistical model selection, focussing on the Akaike Information Criterion (AIC, \citealt{Akk74}) and the so-called  Bayesian Information Criterion (BIC, \citealt{Sch78}). The authors note that in application, adoption of different information criteria can result in the selection of different ``optimal'' models, yet it is generally unclear which criterion should be favoured. They further note that the choice of the most appropriate information criterion is problem-dependent, influenced by one or more of the underlying data-generating process, the nature of the postulated model forms, sample size and model performance criterion. For a Bayesian inference generating a sample from the joint posterior distribution of estimated model parameters, the Divergence Information Criterion (DIC, \citealt{SpgEA02}, \citealt{GlmEA04}) and the Widely Applicable Information Criterion (WAIC, \citealt{Wtn13},\citealt{VhtEA17}) are often used. In comparing AIC and BIC, \cite{ZhnEA23} notes that AIC tends to select more complex models, but that it is not generally possible to foresee which of AIC or BIC would yield models with best out-of-sample predictive performance for a particular model selection problem. Indeed, the authors recommend performing a study involving direct quantification of out-of-sample predictive performance using cross-validation, to quantify the relative performance of different information criteria on problems of the relevant type, as a rational basis for selecting the most appropriate criterion for that problem type. This suggestion was adopted by us in the current work to assess which of a range of criteria based on AIC, BIC, DIC and WAIC yields best performance in a specific extreme value prediction problem involving relatively small samples of CMIP6 climate model output for \TA, below. The earlier article of \cite{GlmEA14} arrives at a similar conclusion regarding predictive information criteria for Bayesian models, including AIC, BIC, DIC and WAIC. The authors state that none of AIC, BIC, DIC and WAIC performs well universally: that AIC is poor in settings with prior information, that DIC is poor when the posterior distribution is not well summarised by its mean, and that WAIC relies on data partition and cross-validation, themselves problematic procedures in the presence of dependence. The authors lean towards cross-validation as their favoured approach. \cite{Kim17} describes a simulation study to assess the relative performance of AIC, the corrected AIC (\citealt{HrvTsa89}), BIC and the likelihood ratio test (LRT) in identifying underlying stationary and non-stationary models with differing characteristics, from samples of varying sizes. The authors note that AIC tends to perform better for small samples (sample size <40), whereas BIC and LRT performance is better for larger samples. The driver of this difference in performance is that AIC tends to select more complex models than BIC and LRT.
	
	We note that many other information criteria for model selection have been proposed and are used, including minimum description length (MDL, \citealt{Rss78}; related to BIC), the risk inflation criterion (RIC, \citealt{FstGrg94}; with an even stronger model complexity penalty than BIC, used in high-dimensional settings), and the Hannan–Quinn Information Criterion (HQIC, \citealt{HnnQnn79}; used in time series modelling).
	
	\subsection{GEV regression for extreme temperatures} \label{SM:Ltr:GEVR}
	In a non-stationary extreme value setting, generalised extreme value (GEV) regression is often used to relate variation of block maxima of some environmental variable with respect to covariates. In the current work, we apply parametric GEV regression to understand temporal changes in the distribution of annual maxima of \TA. In related work, \cite{KhrZwr05} uses parametric GEV regression, with linear variation of all GEV parameters in time, to quantify non-stationarity of annual maxima of various temperature indices. The regression is estimated using L-moments and maximum likelihood, and bootstrapping employed to provide a quantification of uncertainty. The authors show that spatially-averaged parameter estimates for GEV shape and scale show little change in time, whereas increases in temperature extremes can be predominantly explained by increases in the GEV location parameter: that is, global changes in temperature extremes tend to be associated primarily with the overall shift of distribution of annual extremes towards a warmer mean climate, and with only relatively small changes in the actual shape of the extreme temperature distribution. Changes in the distribution of extreme precipitation are more intricate. \cite{ZwrEA11} also uses GEV regression, now with non-stationary GEV location only, to quantify the influence on long return period daily temperature extremes at regional scales. \cite{KhrEA13} again uses GEV regression to update the analysis of \cite{KhrZwr05} for CMIP5 model outputs, estimated using both L-moments and maximum likelihood. Now, GEV location and scale are assumed to vary linearly in time, but GEV shape assumed time-invariant. \cite{KhrEA18} is a further follow-up paper, comparing CMIP5 and CMIP6 return values. \cite{LiEA21} examines annual extremes of daily temperature from CMIP6 models, by fitting stationary GEV models independently to each interval of a partition of the time domain into consecutive blocks. This is done, since the authors claim that it is not possible to fit non-stationary GEV models reliably to time series of climate model output with short length; we hope that the current work demonstrates that this claim is generally not true. \cite{AbdPpl23} use a mixture of model selection information criteria, including AIC, BIC and the Anderson-Darling statistic, to select models for extreme precipitation in CMIP6 projections. Models considered involve linear representations for GEV regression location and scale. No conclusions are made about the best choice of information criterion to use in their study; the output of all criteria are used for model selection, but details are not given. 
	
	\subsection{Related literature} \label{SM:Ltr:Oth}
	A number of software packages for R and other programming languages provide functionality for parametric and non-parametric GEV regression (see e.g. \citealt{BlzEA23}).  \cite{DiNing23} use a bootstrap procedure for variable selection in GEV regression. \cite{PhtEA10} adopt a variable selection approach first proposed by \cite{Kvr08}, incorporating a prior specification favouring sparse covariate descriptions, to characterise the covariate dependence of the location parameter in a GEV regression. \cite{FlkEA24} use BIC to select physical covariates in non-stationary extreme value models of flood frequency in England and Wales. They note however that AIC may be a useful information criterion when taking a ``more nuanced view of model selection''.  The python software developed for the scenario-coupled parametric GEV regression analysis is available via GitHub (at \citealt{LchJnt26}).
	
	In a semi-parametric GEV regression setting, \cite{NsrEA13} report a B-spline model for extreme U.S. rainfall. \cite{Grd23} proposes the use of Bayesian P-splines to characterise the non-linear effects of covariates on GEV parameters for samples of annual maxima of river discharge. Choice of functional form for covariate dependence is achieved using a grouped horseshoe prior to encourage shrinkage of non-relevant covariates. \cite{RchHsr26} model spatio-temporal extremes of wildfires using neural networks. In the related field of non-stationary peaks over threshold modelling, there are numerous examples of non-stationary non-parametric generalised Pareto regression in the environmental and engineering literature (see e.g. \citealt{JnsEA15}, \citealt{RndEA15a}). More generally, \cite{LeeEA15} propose the use of Bayesian measures of surprise to determine suitable thresholds for extreme value models. These quantify the level of support for the proposed extremal model and threshold, without the need to specify any model alternatives, and allow direct comparison of competing threshold candidates with different numbers of threshold exceedances. \cite{MtrRdd25} describes a tool for sample size determination in stationary GEV fitting for climate applications, to ensure that estimates of extreme quantiles are obtained with the required precision. 
	
	A number of authors have explored different aspects of Bayesian inference in a parametric GEV regression setting. For example, \cite{FrdThr12} use the method of \cite{Hff09} for Bayesian covariate selection in GEV regression. \cite{CstEA23} note that covariate selection in GEV regression is generally challenging, and use stochastic search variable selection for the selection of atmospheric covariates in modelling annual maximum temperature series for locations in Spain using GEV regression. \cite{AldEA23} examine whether the concentration of atmospheric carbon dioxide explains variation in the distribution of annual maximum daily maximum temperature in Europe. Model selection is performed using a hold-out sample with respect to various scoring rules for probabilistic forecasts, and AIC. The authors find good agreement in optimal model choice (from five candidates, with different combinations of no trends or of linear trends in GEV location and scale) across the scoring rules and AIC. \cite{PrnVht17} provides a comparison of Bayesian predictive methods for model selection. 
	
	%%%%%%%%%%%%%%%%%%%%%%%%%%%%%%%%%%%%%%%%%%%%%%%%%%%%%%%%%%%%%%%%%%
	\clearpage
	\FloatBarrier
	\section{Illustrations of regional annual maxima and minima time series} \label{SM:TS}
	%%%%%%%%%%%%%%%%%%%%%%%%%%%%%%%%%%%%%%%%%%%%%%%%%%%%%%%%%%%%%%%%%%
	
	\begin{figure}[!ht]
		\centering
		\includegraphics[width=1\textwidth]{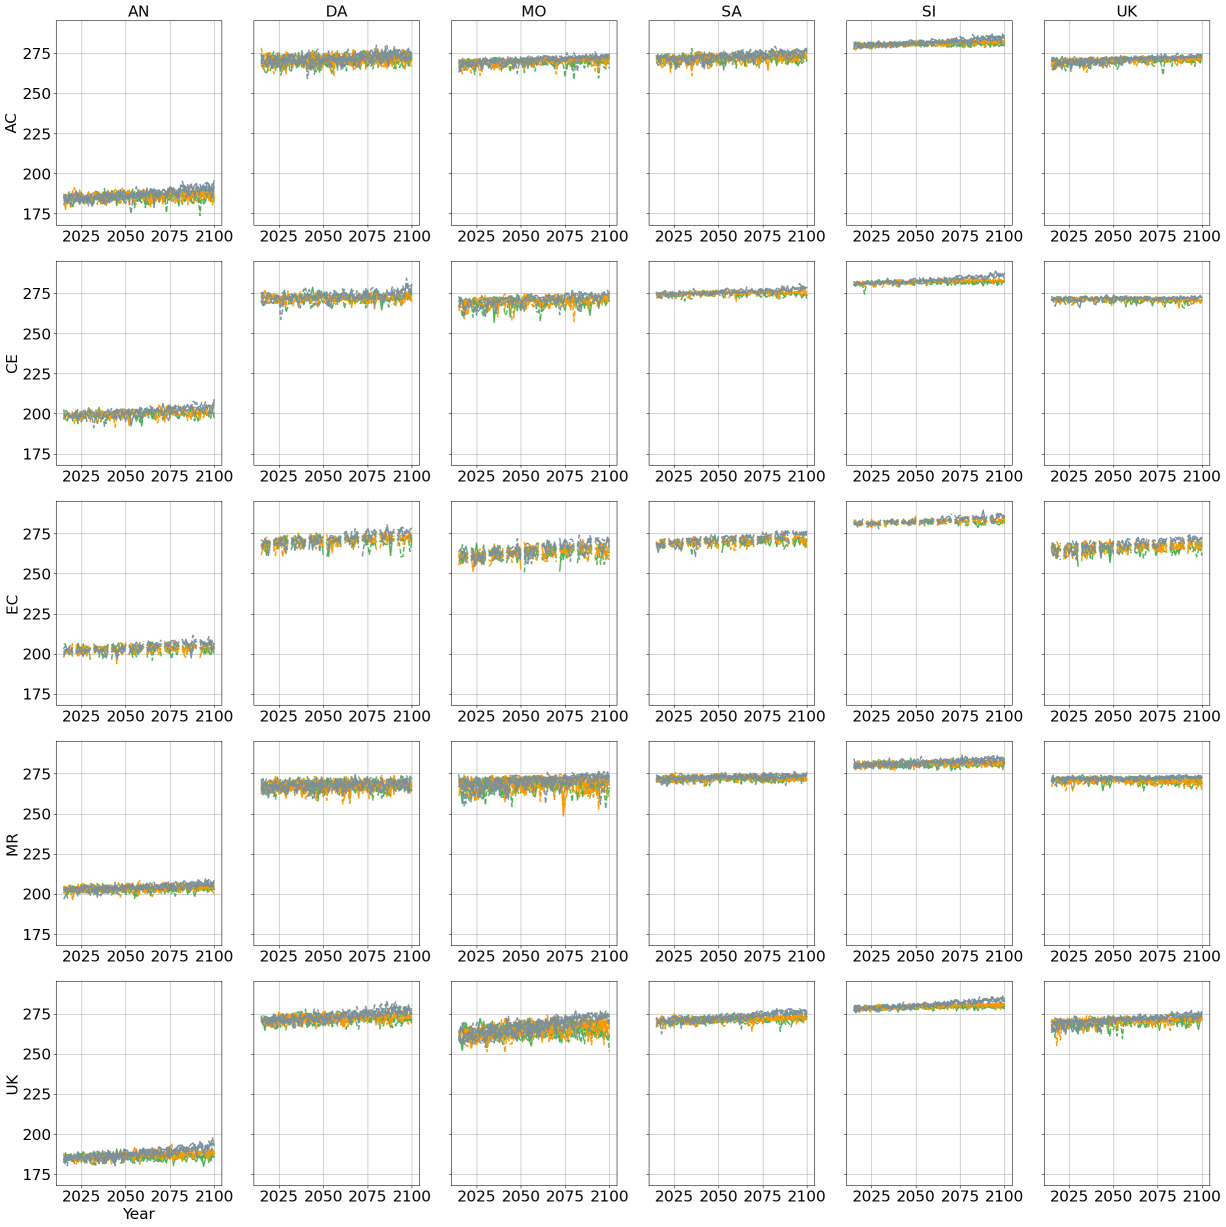}
		\caption{Time series of regional annual minima of \TA (K) by GCM (rows: \AC, \CE, \EC, \MR and \UK) and region (column: : \DAN, \DDA, \DMO, \DSA, \DSI and \DUK). In each panel, climate scenarios are distinguished by colour: \SL (green), \SM (orange), \SM (grey). Climate ensemble runs for each scenario are distinguished by line style. Corresponding spatial annual maxima time series are given in Figure~3 of the main text.} 
		\label{Fgr-Mnm-TS-LctxGcm}
	\end{figure}

	%%%%%%%%%%%%%%%%%%%%%%%%%%%%%%%%%%%%%%%%%%%%%%%%%%%%%%%%%%%%%%%%%%
	\clearpage
	\FloatBarrier
	\section{Bayesian inference} \label{SM:MCMC}
	%%%%%%%%%%%%%%%%%%%%%%%%%%%%%%%%%%%%%%%%%%%%%%%%%%%%%%%%%%%%
	%
	Inference for the GEV regression models described in Section~3.2 is performed using Markov chain Monte Carlo (MCMC, see e.g. \citealt{GmrLps06}) following the method of \cite{RbrRsn09}. This procedure was reported previously in \cite{EwnJnt23a}, but is summarised here for completeness and ease of reference. All the parameters $\boldsymbol{\theta}$ of the model are jointly updated for a sequence of $n_B+n_S$ MCMC iterations. At each iteration, a new set of parameter values is proposed, and accepted according to the Metropolis-Hastings acceptance criterion based on (a) the sample likelihood evaluated at the current and candidate states, and (b) the values of the prior densities for parameters at the current and candidate states. Following $n_B$ burn-in iterations, the Markov chain is judged to have converged, so that the subsequent $n_S$ iterations provide a valid sample from the joint posterior distribution of parameters. Prior distributions were specified as follows: $\xi \sim U(-1,0.2)$; $\sigma \sim U(0,\infty)$; $\mu \sim U(-\infty, \infty)$. Likelihoods for the models are available from the distributions given in the main text. An appropriate starting solution $\boldsymbol{\theta}_1$ for the MCMC inference was obtained by random sampling from the prior distributions of parameters, ensuring a valid likelihood. 
	
	For the first $n_S<n_B$ iterations, candidate parameter values $\boldsymbol{\theta}_k^c$ are proposed (independently) from $\boldsymbol{\theta}_k^c \sim N(\boldsymbol{0},0.1^2 \boldsymbol{I})$ following \cite{RbrRsn09}. Thereafter $\boldsymbol{\theta}_k^c \sim (1-\beta) N\left(\boldsymbol{\theta}_{k-1}, 2.38^{2} \Sigma_{k}\right)+\beta N\left(\boldsymbol{\theta}_{k-1}, 0.1^{2} / 4\right)$, where $\beta=0.05$, $\Sigma_{k}$ is the empirical variance-covariance matrix of parameters from the past $k$ iterations, and $\boldsymbol{\theta}_{k-1}$ is the current value of parameters. Throughout, a candidate state is accepted using the standard Metropolis-Hastings acceptance criterion. Since prior distributions for parameters are uniform, and proposals symmetric, this criterion is effectively just a likelihood ratio. That is, we accept the candidate state with probability $\min (1, L(\boldsymbol{\theta}^c)/L(\boldsymbol{\theta}))$, where $L(\boldsymbol{\theta})$ and $L(\boldsymbol{\theta}^c)$ are the likelihoods evaluated at the current and candidate states respectively, with candidates lying outside their prior domains rejected.
	
	%%%%%%%%%%%%%%%%%%%%%%%%%%%%%%%%%%%%%%%%%%%%%%%%%%%%%%%%%%%%%%%%%%
	\clearpage
	\FloatBarrier
	\section{Results for regional annual maxima} \label{SM:Mxm}
	%%%%%%%%%%%%%%%%%%%%%%%%%%%%%%%%%%%%%%%%%%%%%%%%%%%%%%%%%%%%%%%%%%
	
	\foreach \lct/\lctv in {AN/\DAN, DA/\DDA, MO/\DMO, SA/\DSA, SI/\DSI, UK/\DUK} {
		\foreach \gcm/\gcmv in {AC/\AC, CE/\CE, EC/\EC, MR/\MR, UK/\UK} {
			\begin{figure}[!ht]
				\centering
				\includegraphics[width=1\textwidth]{Mxm-Lct\lct-Gcm\gcm.png}
				%\caption{Mxm-Lct\lct-Gcm\gcm}
				\caption{Summary of scenario-coupled GEV regression for regional annual maxima of the \lctv region using \gcmv GCM data. Top left: plots of BIC3 (solid line) and AIC3 (dashed line) for each available ensemble (distinguished by colour, see Table~2 of the main text and legend in bottom-right panel); optimal model choice using BIC3 (AIC3) indicated using red disc (blue cross). Top right: box-whisker plots summarising the distribution of the difference in the 100-year return value between 2025 and 2125 ($\Delta Q_1$; see Equation~7) for climate scenario \SL as a function of fitted model complexity (x-axis) and ensemble (distinguished by colour, with consistent ensemble colouring across panels); location of horizontal centre line of each box indicates posterior median of $\Delta Q_1$; location of top (bottom) side of each box indicates 75\%ile (25\%ile) point, and top (bottom) of whiskers the 97.5\%ile (2.5\%ile) point of the posterior distribution. Bottom left and right: analogues of top right for scenarios \SM ($\Delta Q_2$) and \SH ($\Delta Q_3$). Value of $\Delta Q_j$, $j=1,2,3$ under model CCC is identically zero, and is omitted from bottom panels when convenient to provide better illustration of the variation in estimates under more complex models. For comparison with Figure 6 of the main text.}	
				\label{Mxm-Lct\lct-Gcm\gcm}
			\end{figure}
		}
	}
	
	\begin{figure}[!ht]
		\centering
		\includegraphics[width=1\textwidth]{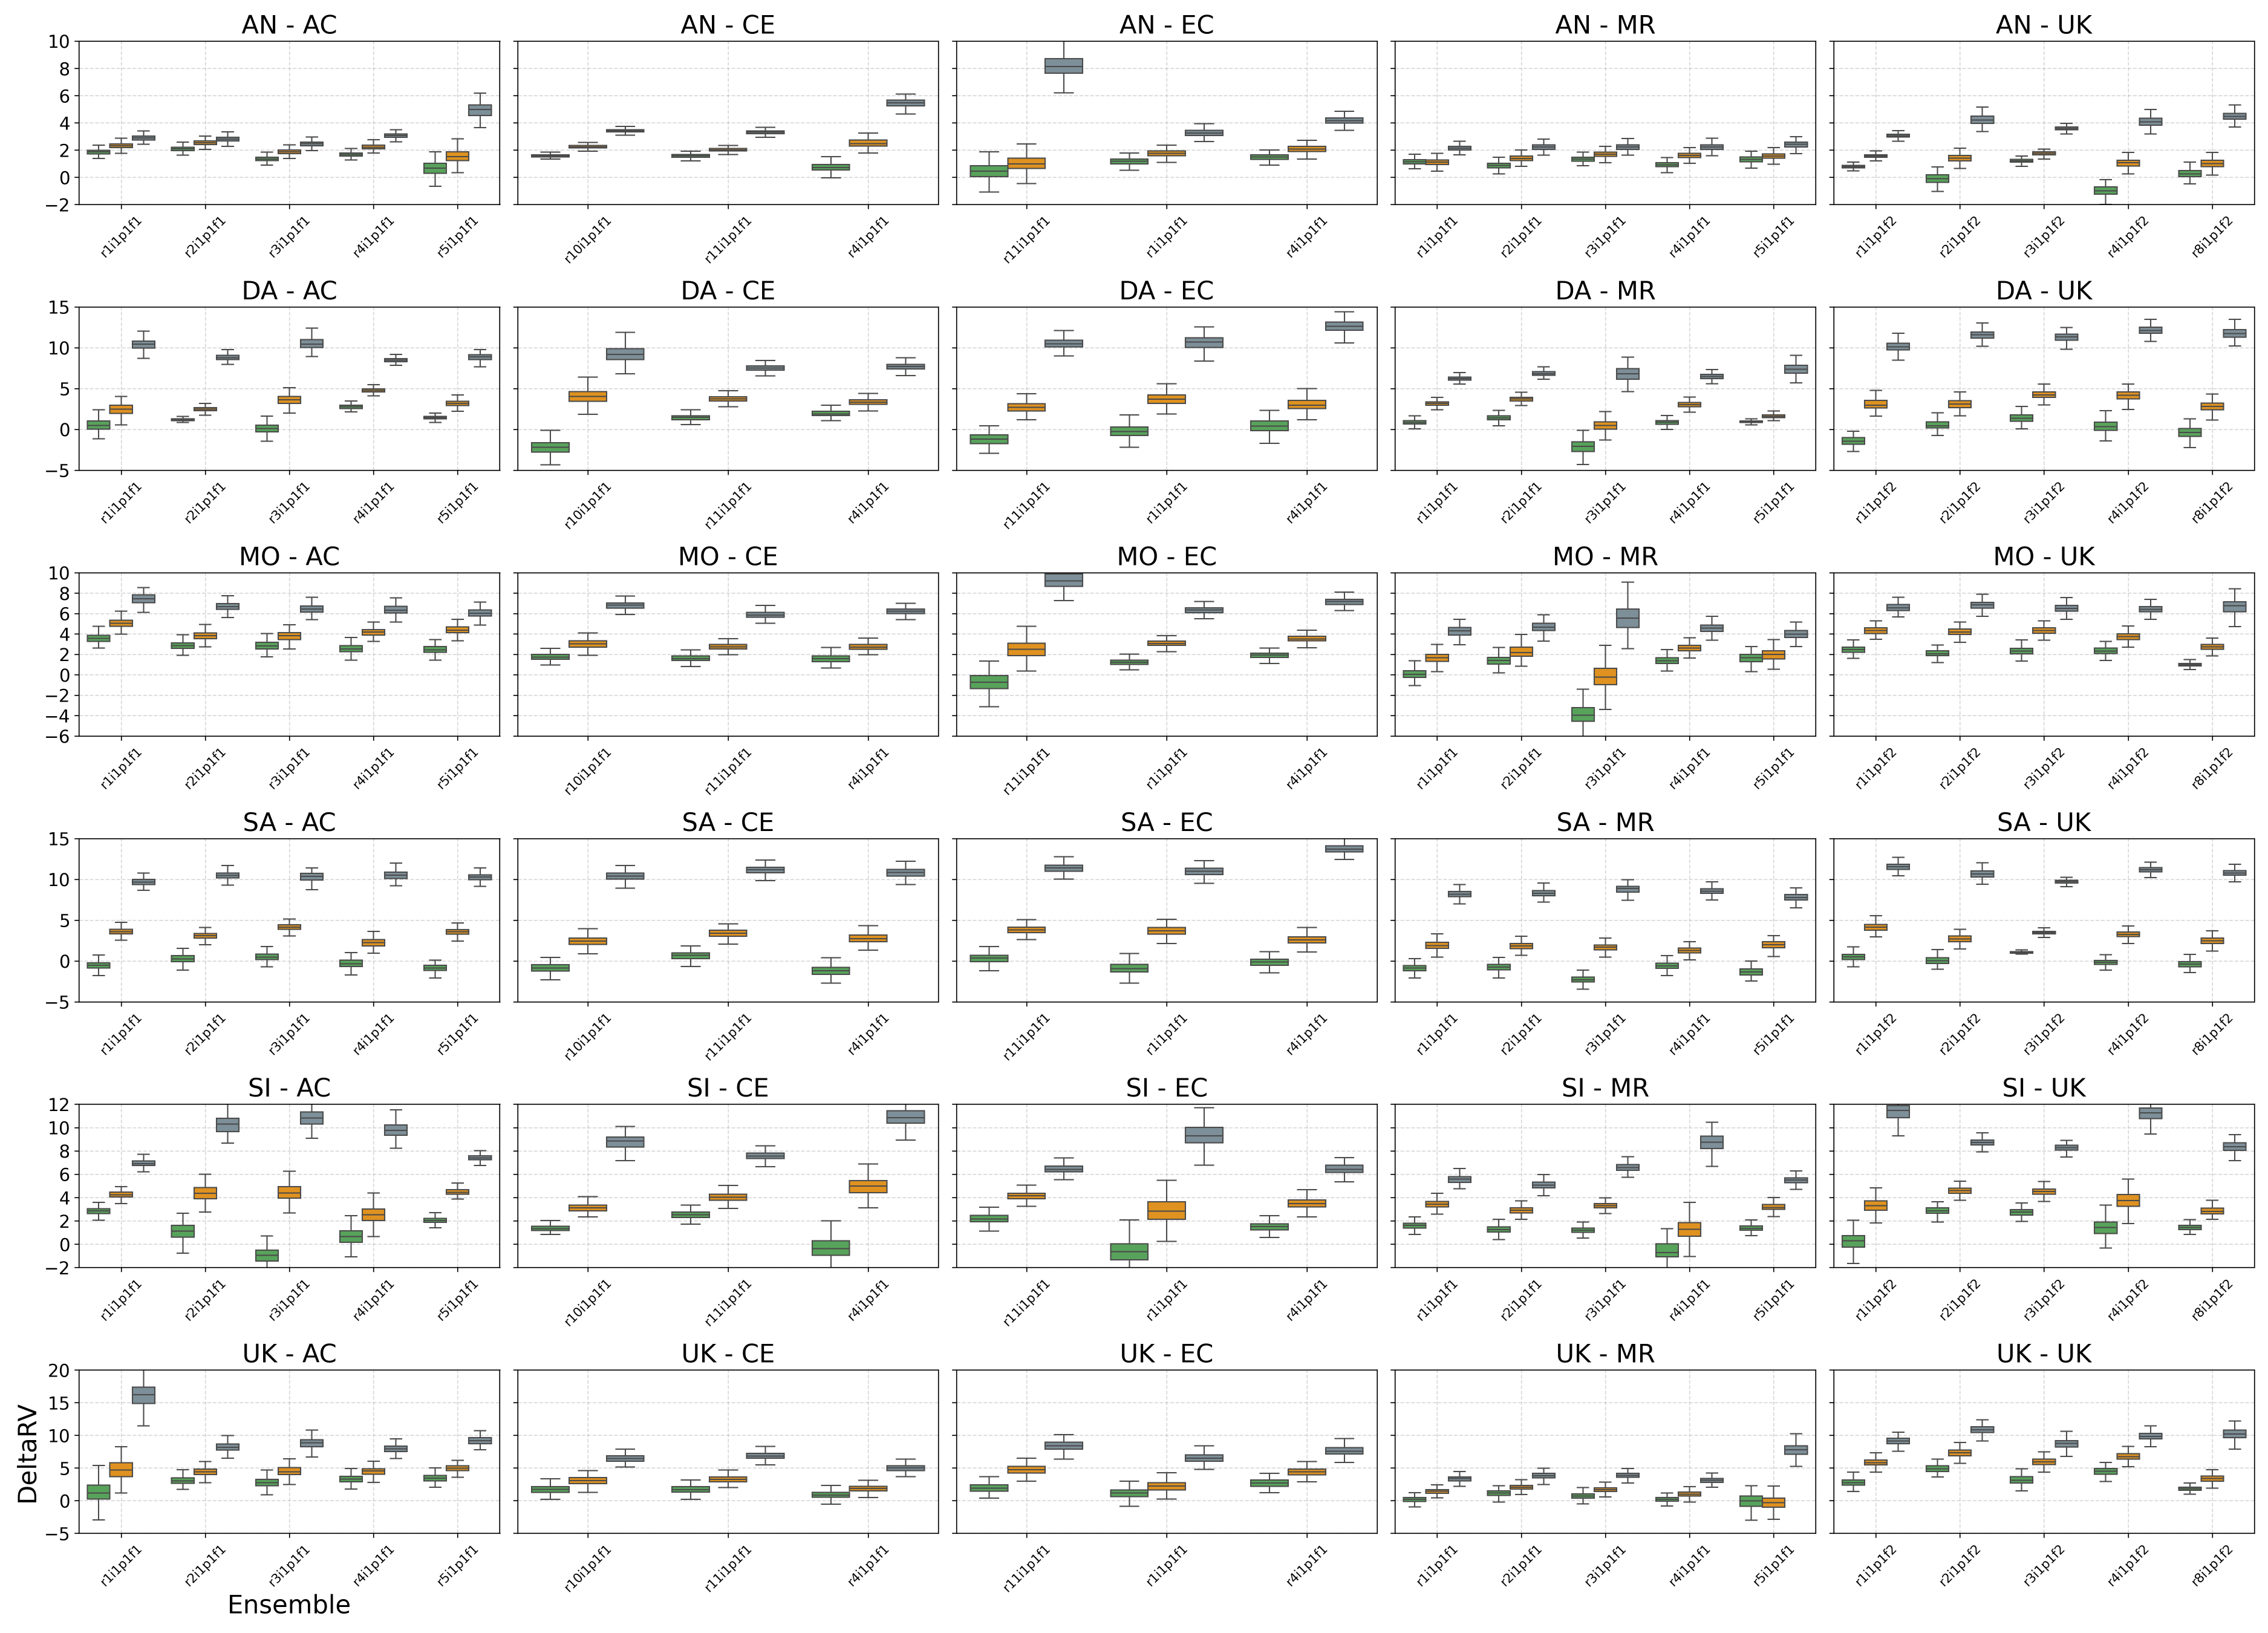}
		\caption{Summary of inferences for return value differences $\Delta Q_j$, $j=1,2,3$ (see Equation~7) of regional annual maxima using BIC3 for model selection. Each panel shows box-whisker plots summarising the posterior distribution of $\Delta Q$ for climate scenarios \SL ($j=1$, green), \SM ($j=2$, orange) and \SH ($j=3$, grey) for each of up to five climate ensembles. Different panels show inferences for specific combinations of regions and locations; see Tables 1 and 2 for region and GCM acronyms.} 
		\label{Fgr-Mxm-BW-LctGcmScn-Ens-BIC}
	\end{figure}
	
	\begin{figure}[!ht]
		\centering
		\includegraphics[width=1\textwidth]{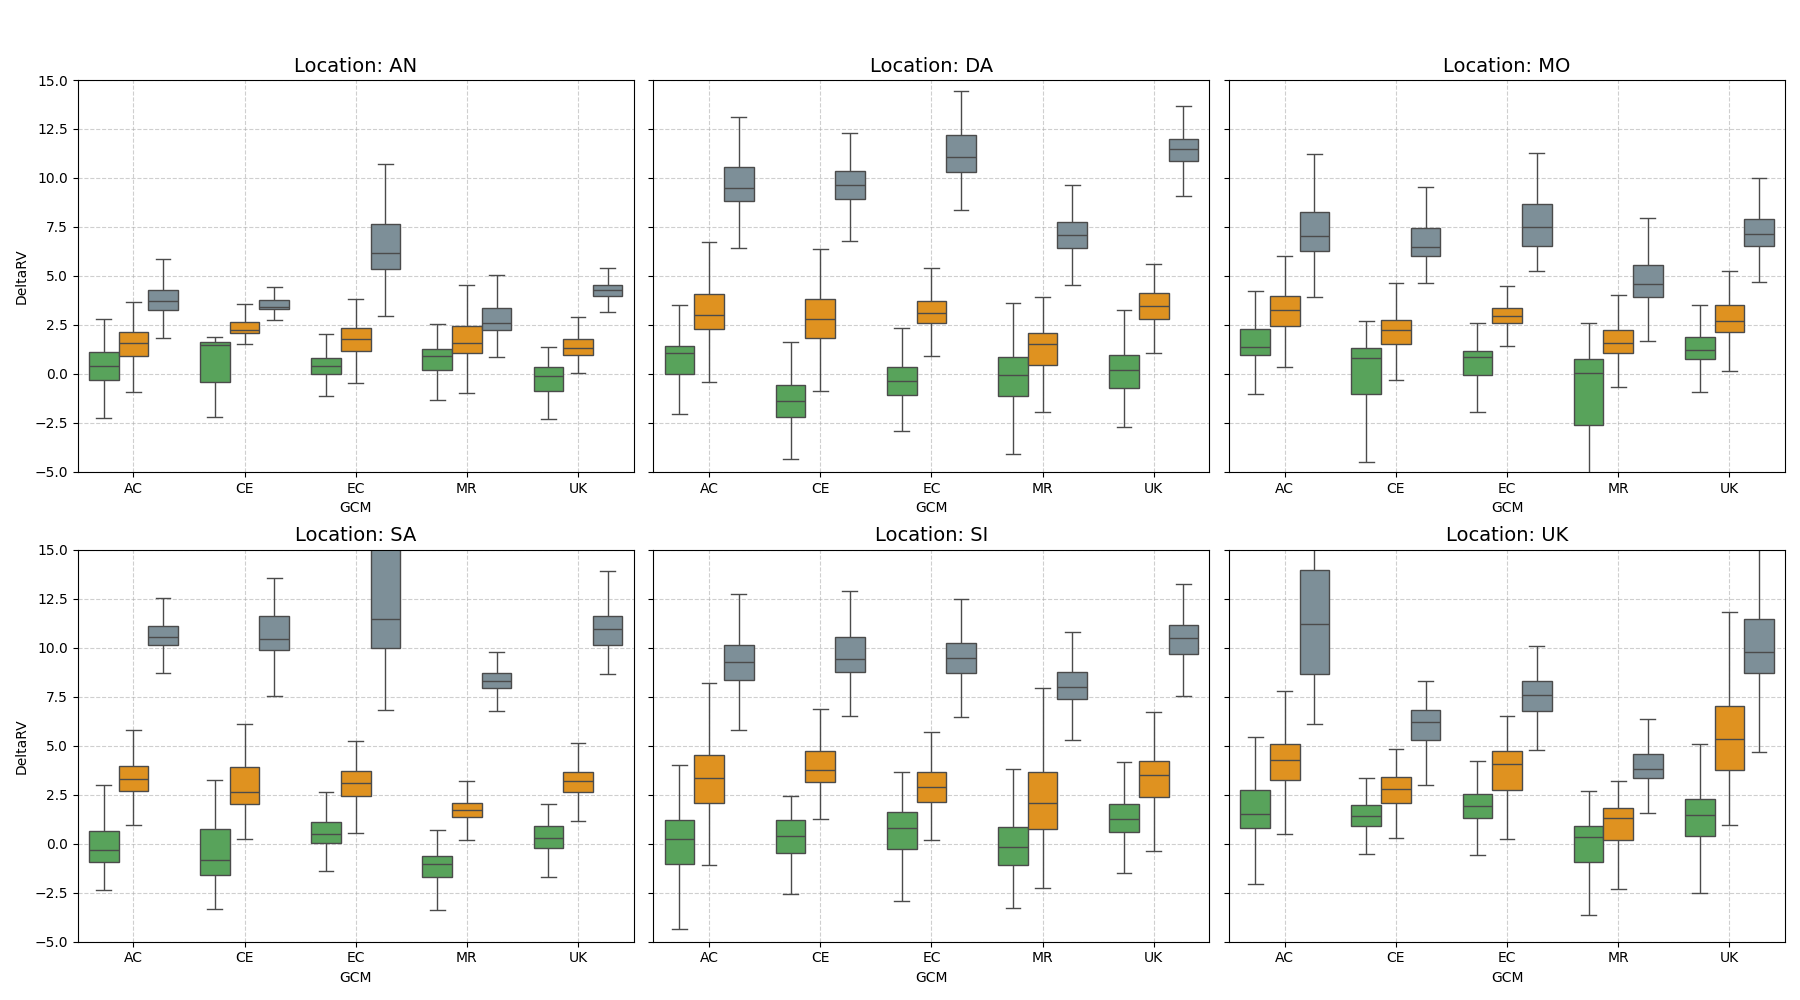}
		\caption{Summary of inferences for return value differences $\Delta Q_j$, $j=1,2,3$ (see Equation~7) of regional annual maxima using AIC3 for model selection, aggregated over climate ensemble. Each panel shows box-whisker plots summarising the posterior distribution of $\Delta Q$ for climate scenarios \SL ($j=1$, green), \SM ($j=2$, orange) and \SH ($j=3$, grey) and each of five GCMs (\AC, \CE, \EC, \MR, \UK). Left to right, top to bottom, panels show inferences for the \DAN, \DDA, \DMO, \DSA, \DSI and \DUK regions. For comparison with Figure~7.} 
		\label{Fgr-Mxm-BW-LctGcmScn-DIC}
	\end{figure}
	
	\begin{figure}[!ht]
		\centering
		\includegraphics[width=1\textwidth]{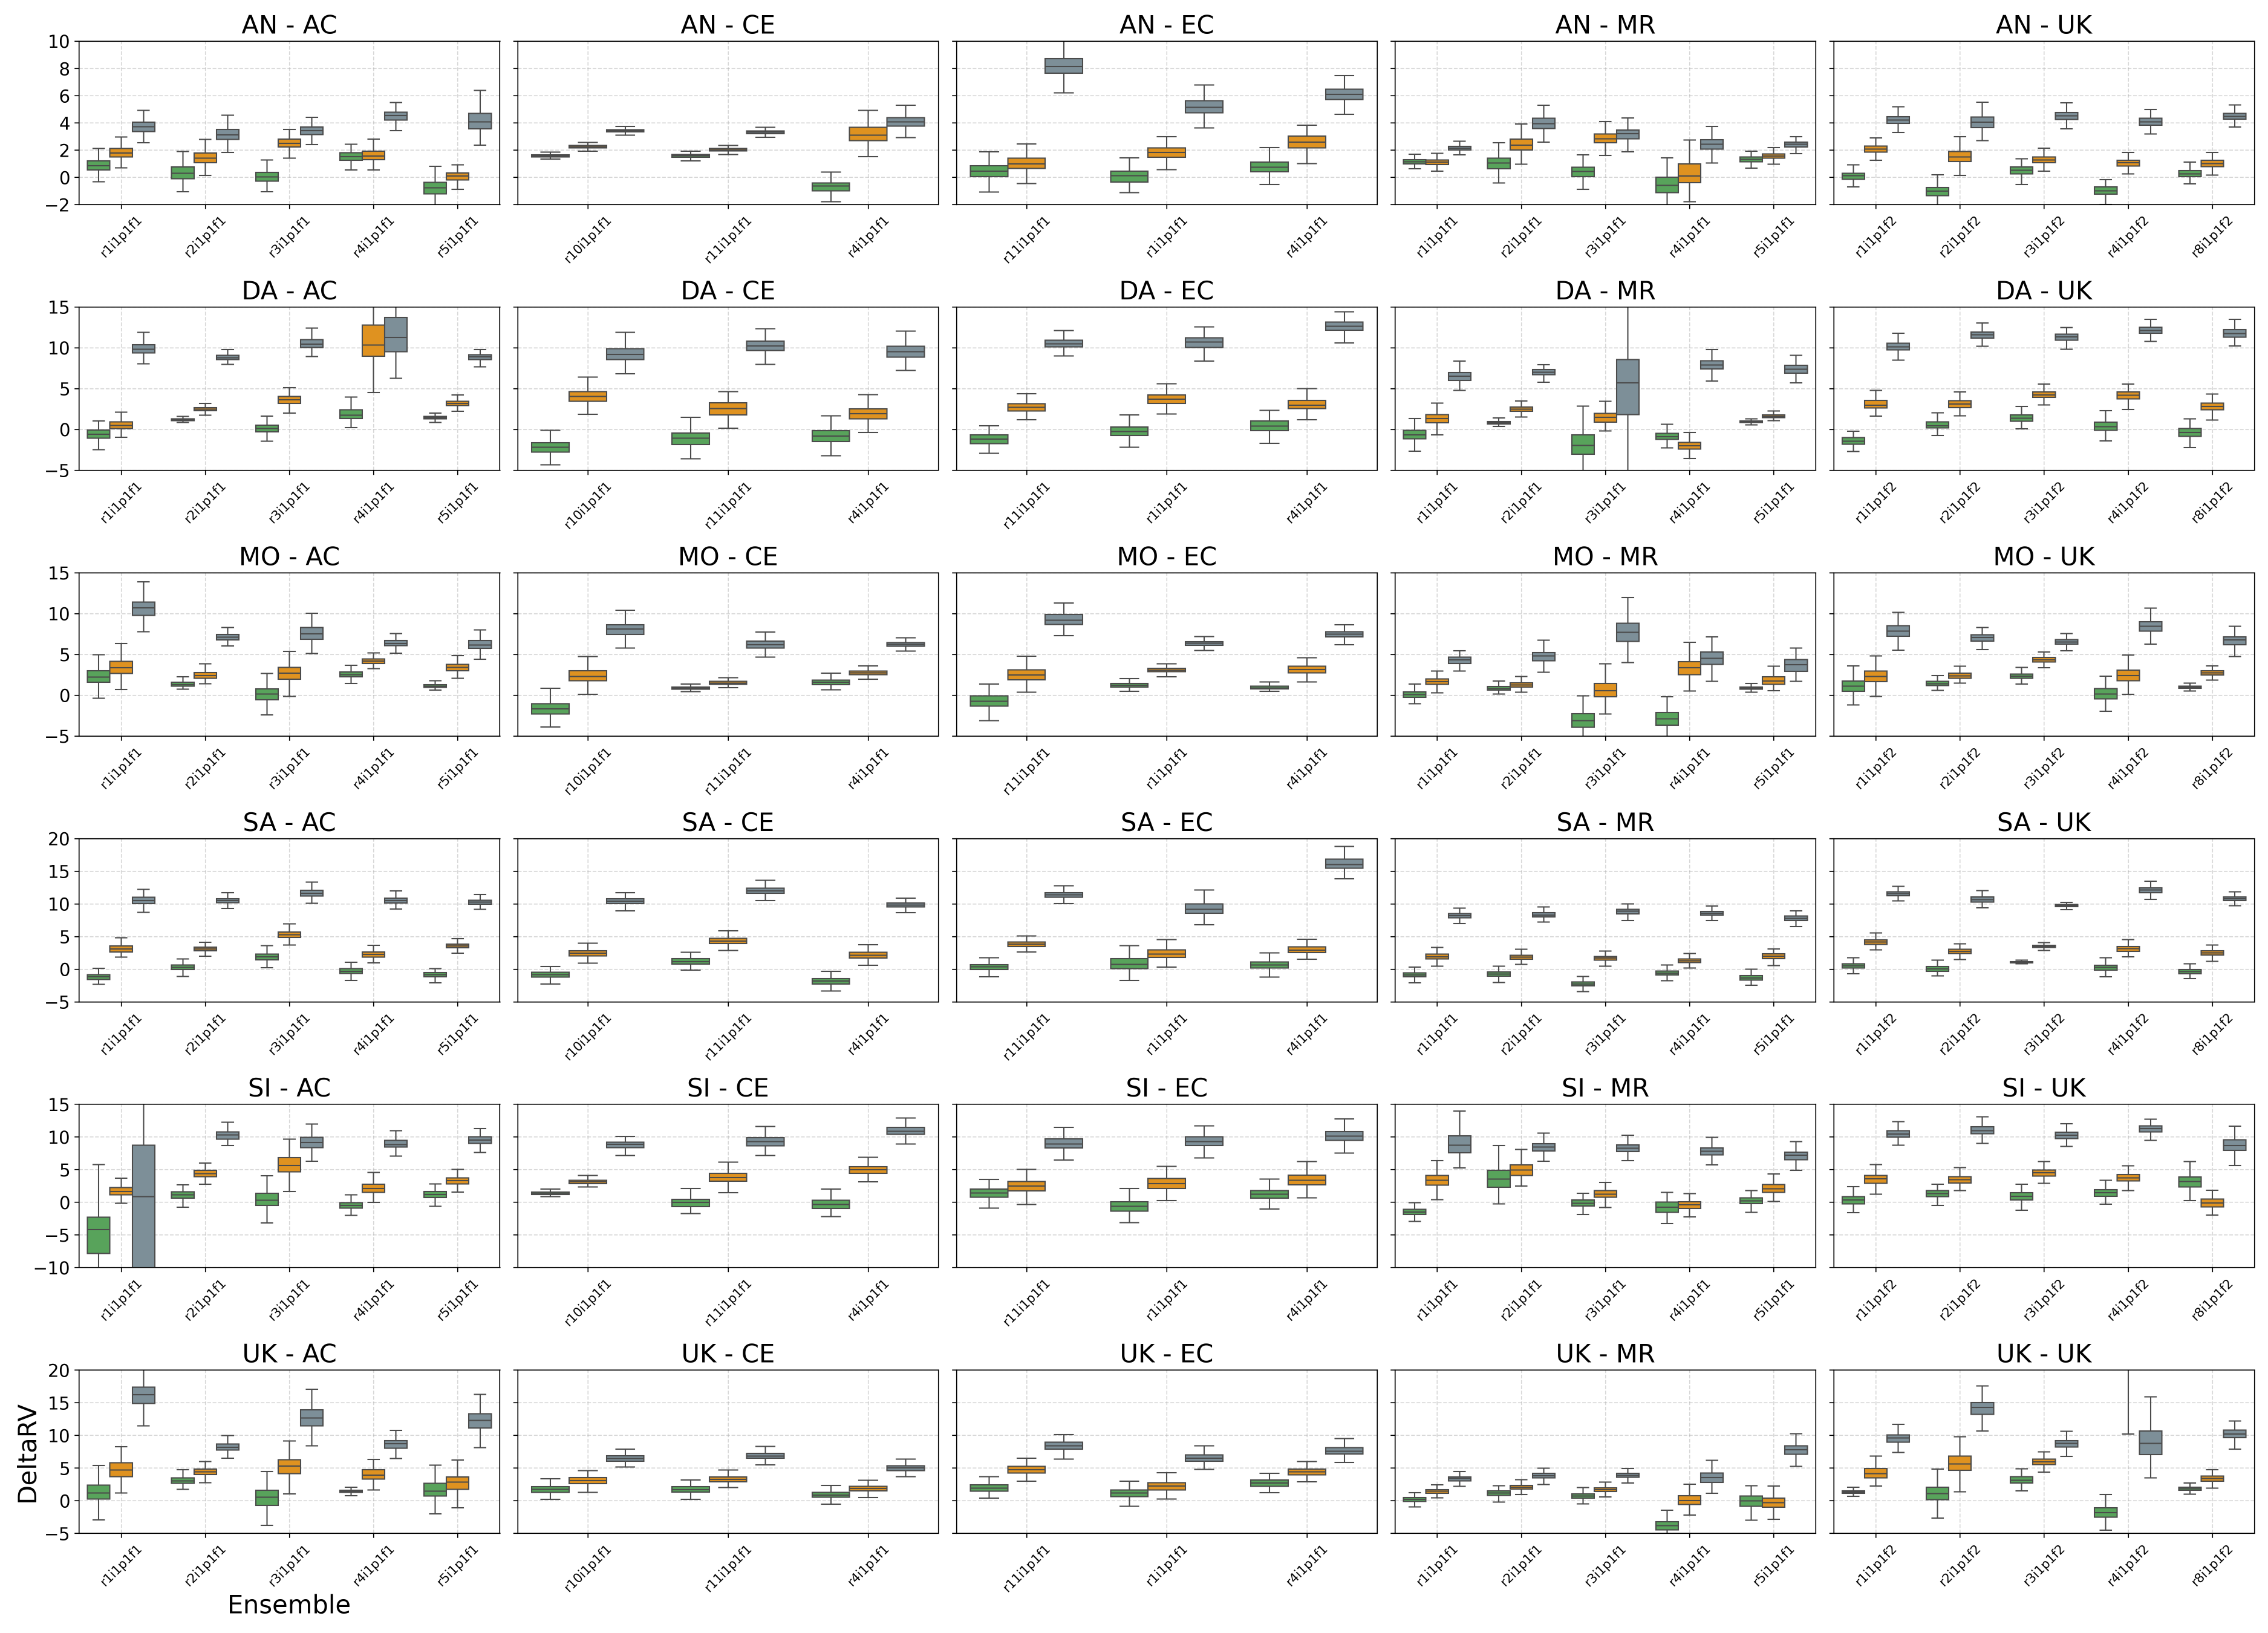}
		\caption{Summary of inferences for return value differences $\Delta Q_j$, $j=1,2,3$ (see Equation~7) of regional annual maxima using AIC3 for model selection. Each panel shows box-whisker plots summarising the posterior distribution of $\Delta Q$ for climate scenarios \SL ($j=1$, green), \SM ($j=2$, orange) and \SH ($j=3$, grey) for each of up to five climate ensembles. Different panels show inferences for specific combinations of regions and locations; see Tables 1 and 2 for region and GCM acronyms.} 
		\label{Fgr-Mxm-BW-LctGcmScn-Ens-DIC}
	\end{figure}
	
	\begin{figure}[!ht]
		\centering
		\includegraphics[width=1\textwidth]{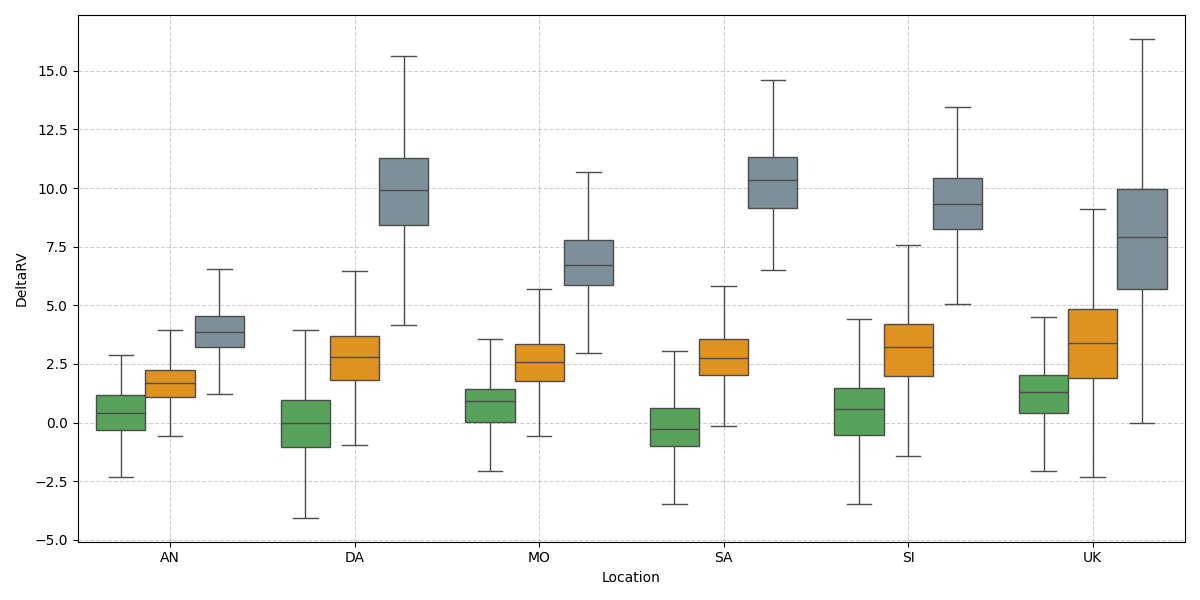}
		\caption{Summary of inferences for return value differences $\Delta Q_j$, $j=1,2,3$ (see Equation~7) of regional annual maxima using AIC3 for model selection, aggregated over climate ensemble and GCM. Box-whisker plots summarise the posterior distribution of $\Delta Q$ for climate scenarios \SL ($j=1$, green), \SM ($j=2$, orange) and \SH ($j=3$, grey) for the \DAN, \DDA, \DMO, \DSA, \DSI and \DUK regions.} 
		\label{Fgr-Mxm-BW-LctScn-DIC}
	\end{figure}
	
	%%%%%%%%%%%%%%%%%%%%%%%%%%%%%%%%%%%%%%%%%%%%%%%%%%%%%%%%%%%%%%%%%%
	\clearpage
	\FloatBarrier
	\section{Results for regional annual minima} \label{SM:Mnm}
	%%%%%%%%%%%%%%%%%%%%%%%%%%%%%%%%%%%%%%%%%%%%%%%%%%%%%%%%%%%%%%%%%%
	
	\foreach \lct/\lctv in {AN/\DAN, DA/\DDA, MO/\DMO, SA/\DSA, SI/\DSI, UK/\DUK} {
		\foreach \gcm/\gcmv in {AC/\AC, CE/\CE, EC/\EC, MR/\MR, UK/\UK} {
			\begin{figure}[!ht]
				\centering
				\includegraphics[width=1\textwidth]{Mnm-Lct\lct-Gcm\gcm.png}
				%\caption{Mxm-Lct\lct-Gcm\gcm}
				\caption{Summary of scenario-coupled GEV regression for regional annual minima of the \lctv region using \gcmv GCM data. Top left: plots of BIC3 (solid line) and AIC3 (dashed line) for each available ensemble (distinguished by colour, see Table~2 of the main text and legend in bottom-right panel); optimal model choice using BIC3 (AIC3) indicated using red disc (blue cross). Top right: box-whisker plots summarising the distribution of the difference in the 100-year return value between 2025 and 2125 ($\Delta Q_1$; see Equation~7) for climate scenario \SL as a function of fitted model complexity (x-axis) and ensemble (distinguished by colour, with consistent ensemble colouring across panels); location of horizontal centre line of each box indicates posterior median of $\Delta Q_1$; location of top (bottom) side of each box indicates 75\%ile (25\%ile) point, and top (bottom) of whiskers the 97.5\%ile (2.5\%ile) point of the posterior distribution. Bottom left and right: analogues of top right for scenarios \SM ($\Delta Q_2$) and \SH ($\Delta Q_3$). Value of $\Delta Q_j$, $j=1,2,3$ under model CCC is identically zero, and is omitted from bottom panels when convenient to provide better illustration of the variation in estimates under more complex models. For comparison with Figure 6 of the main text.}	
				\label{Mnm-Lct\lct-Gcm\gcm}
			\end{figure}
		}
	}
	
	\begin{figure}[!ht]
		\centering
		\includegraphics[width=1\textwidth]{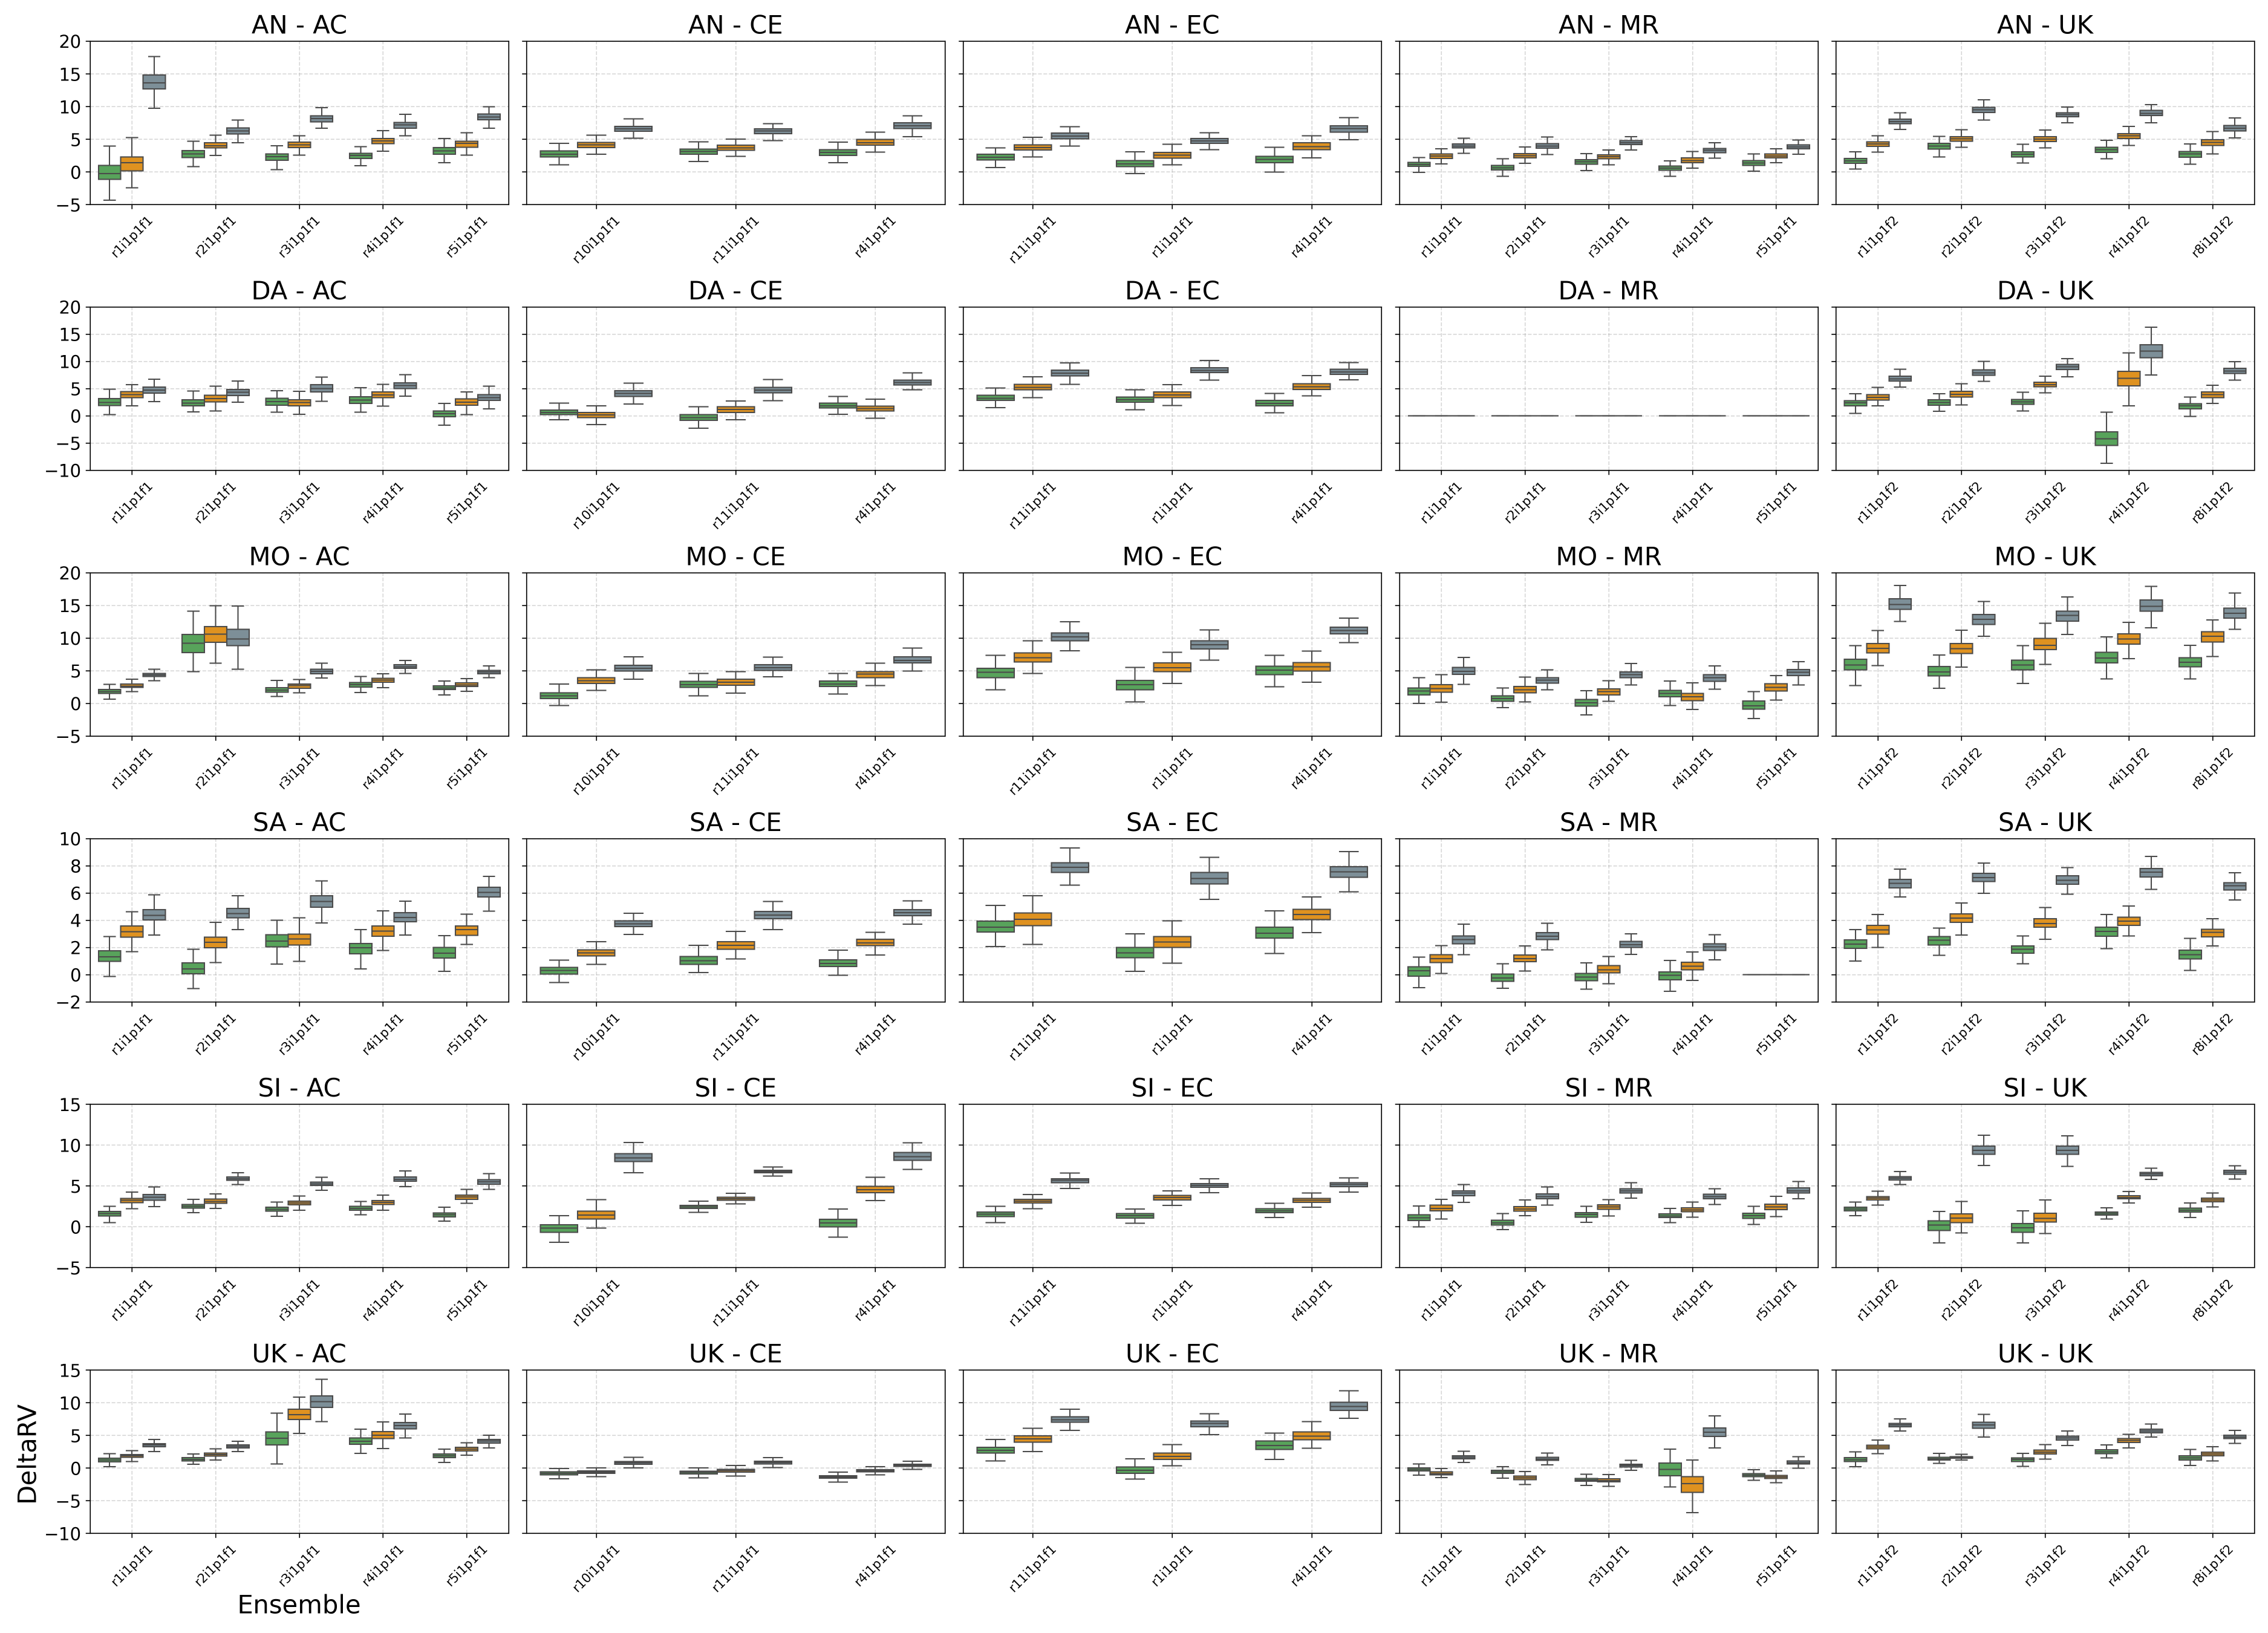}
		\caption{Summary of inferences for return value differences $\Delta Q_j$, $j=1,2,3$ (see Equation~7) of regional annual minima using BIC3 for model selection. Each panel shows box-whisker plots summarising the posterior distribution of $\Delta Q$ for climate scenarios \SL ($j=1$, green), \SM ($j=2$, orange) and \SH ($j=3$, grey) for each of up to five climate ensembles. Different panels show inferences for specific combinations of regions and locations; see Tables 1 and 2 for region and GCM acronyms.} 
		\label{Mnm-BW-LctGcmScn-Ens-BIC}
	\end{figure}
	
	\begin{figure}[!ht]
		\centering
		\includegraphics[width=1\textwidth]{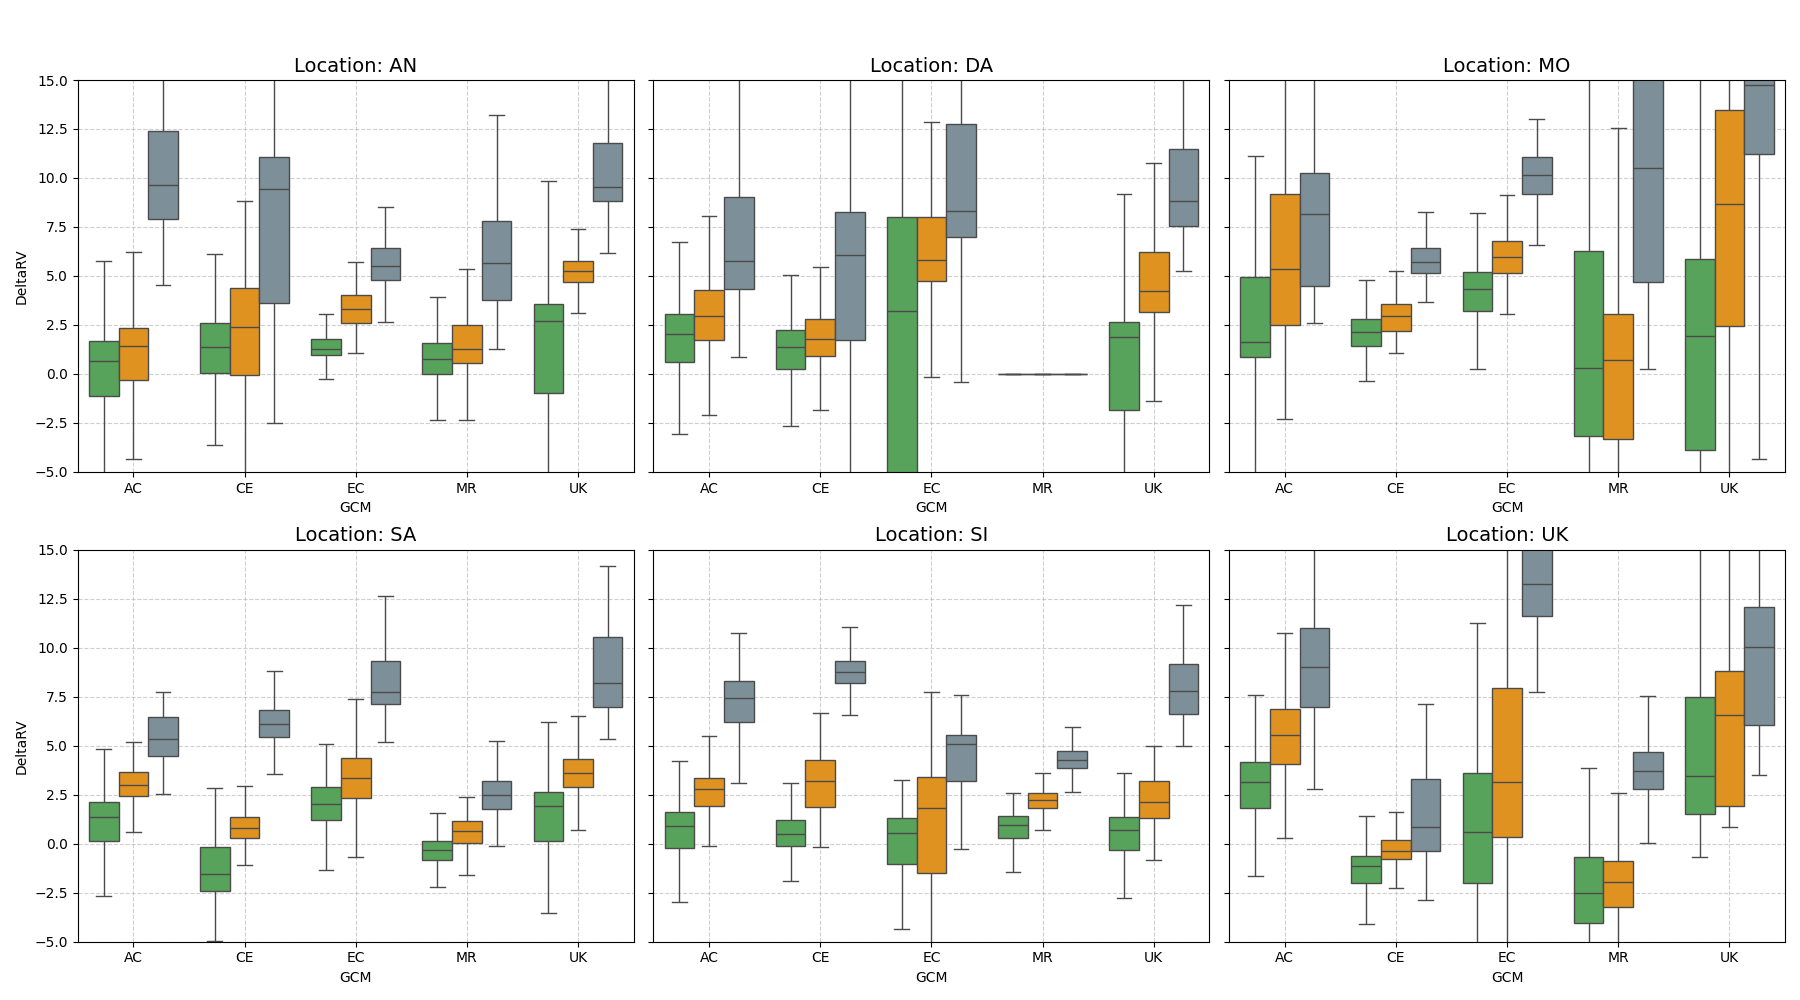}
		\caption{Summary of inferences for return value differences $\Delta Q_j$, $j=1,2,3$ (see Equation~7) of regional annual minima using AIC3 for model selection, aggregated over climate ensemble. Each panel shows box-whisker plots summarising the posterior distribution of $\Delta Q$ for climate scenarios \SL ($j=1$, green), \SM ($j=2$, orange) and \SH ($j=3$, grey) and each of five GCMs (\AC, \CE, \EC, \MR, \UK). Left to right, top to bottom, panels show inferences for the \DAN, \DDA, \DMO, \DSA, \DSI and \DUK regions. For comparison with Figure~10.} 
		\label{Fgr-Mnm-BW-LctGcmScn-DIC}
	\end{figure}
	
	\begin{figure}[!ht]
		\centering
		\includegraphics[width=1\textwidth]{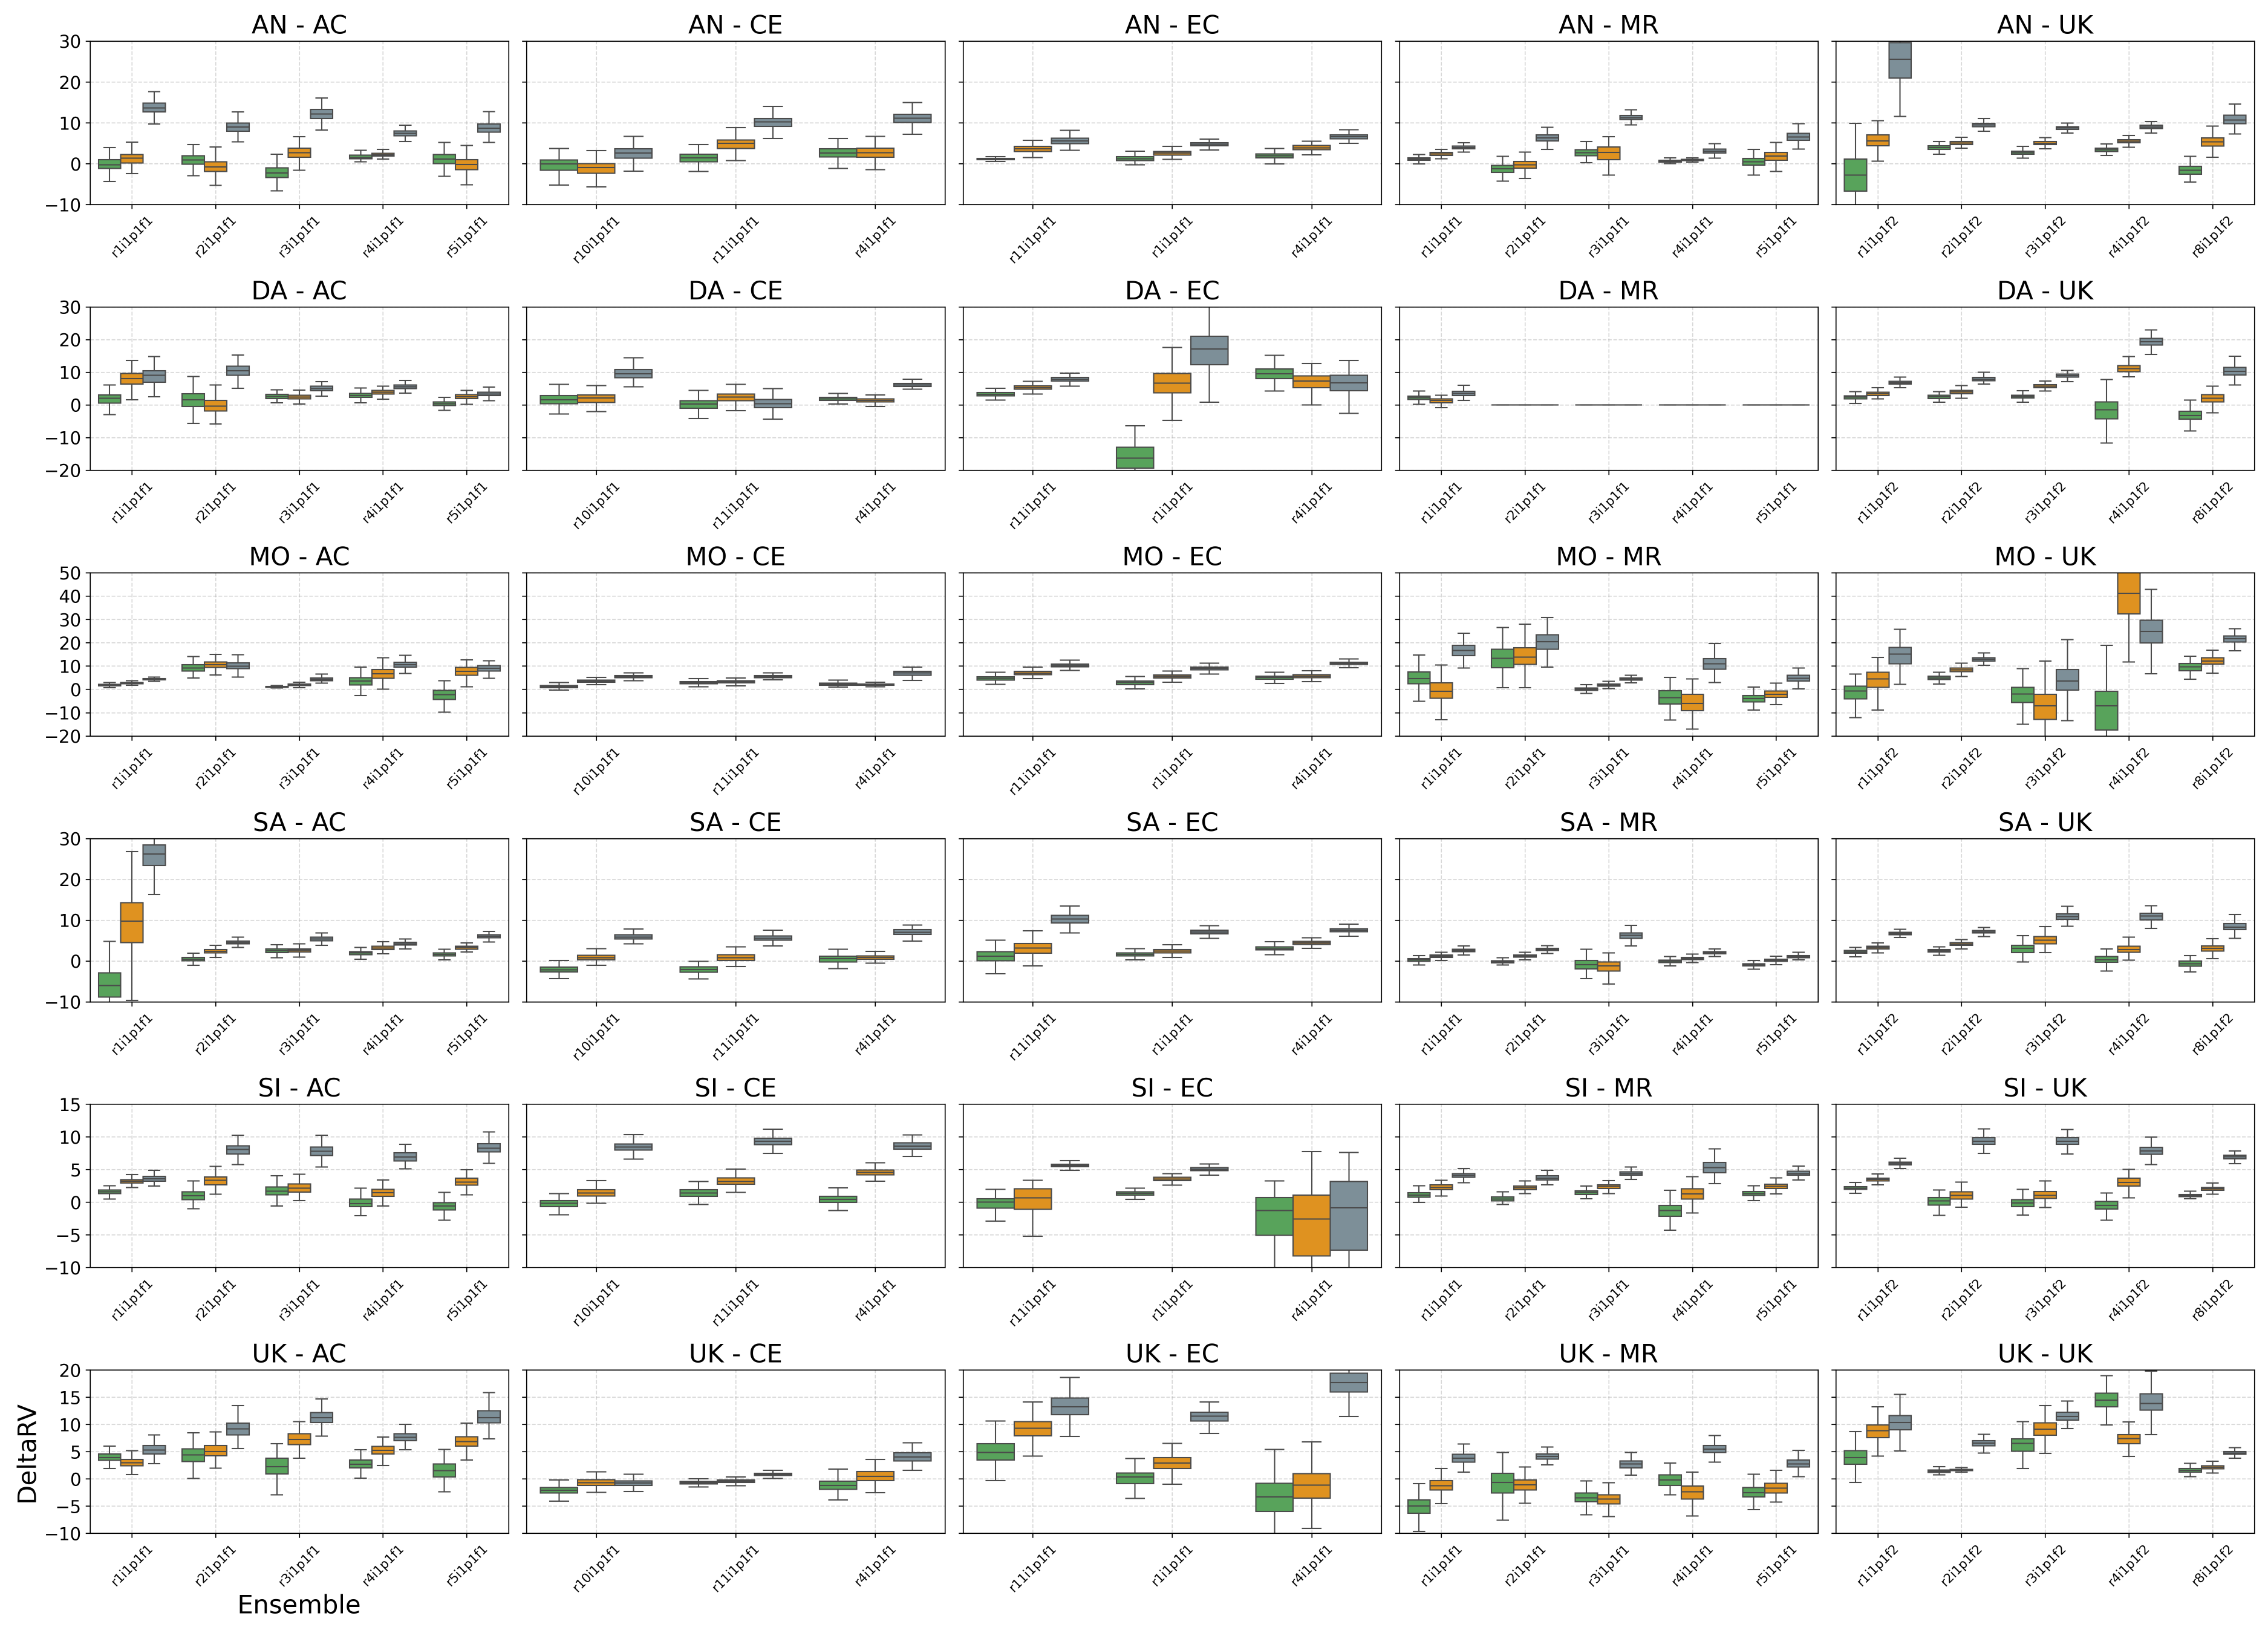}
		\caption{Summary of inferences for return value differences $\Delta Q_j$, $j=1,2,3$ (see Equation~7) of regional annual minima using AIC3 for model selection. Each panel shows box-whisker plots summarising the posterior distribution of $\Delta Q$ for climate scenarios \SL ($j=1$, green), \SM ($j=2$, orange) and \SH ($j=3$, grey) for each of up to five climate ensembles. Different panels show inferences for specific combinations of regions and locations; see Tables 1 and 2 for region and GCM acronyms.} 
		\label{Mnm-BW-LctGcmScn-Ens-DIC}
	\end{figure}
	
	\begin{figure}[!ht]
		\centering
		\includegraphics[width=1\textwidth]{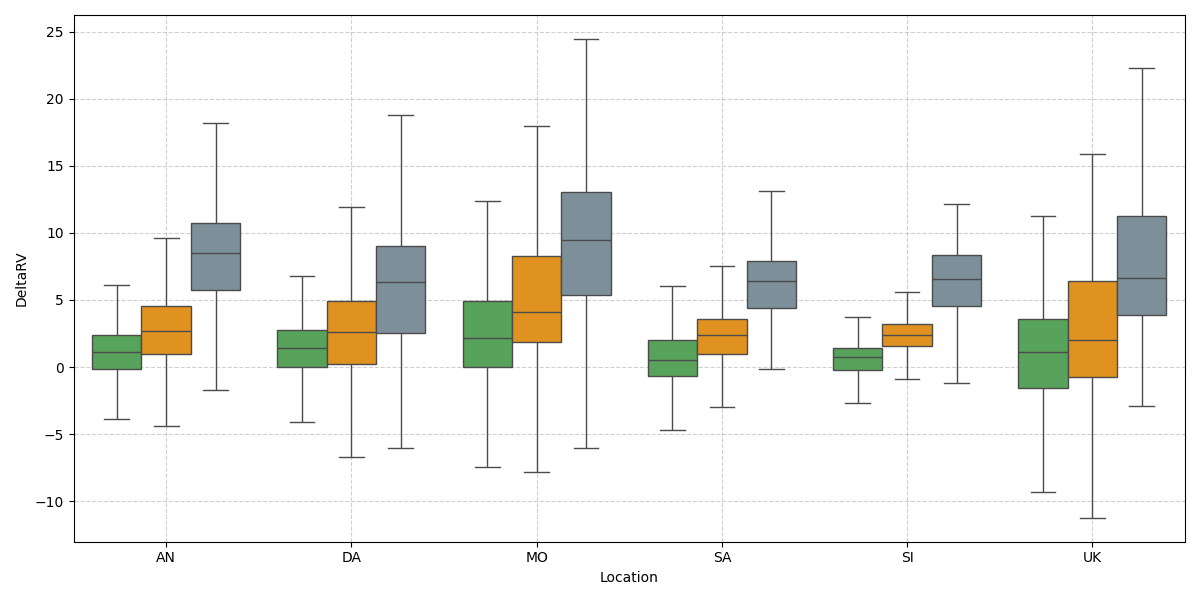}
		\caption{Summary of inferences for return value differences $\Delta Q_j$, $j=1,2,3$ (see Equation~7) of regional annual minima using AIC3 for model selection, aggregated over climate ensemble and GCM. Box-whisker plots summarise the posterior distribution of $\Delta Q$ for climate scenarios \SL ($j=1$, green), \SM ($j=2$, orange) and \SH ($j=3$, grey) for the \DAN, \DDA, \DMO, \DSA, \DSI and \DUK regions.} 
		\label{Fgr-Mnm-BW-LctScn-DIC}
	\end{figure}
	
	%%%%%%%%%%%%%%%%%%%%%%%%%%%%%%%%%%%%%%%%%%%%%%%%%%%%%%%%%%%%%%%%%%
	\clearpage
	\FloatBarrier
	\section{Differences between changes in return value for maxima and minima} \label{SM:MxmMnmDff}
	%%%%%%%%%%%%%%%%%%%%%%%%%%%%%%%%%%%%%%%%%%%%%%%%%%%%%%%%%%%%%%%%%%
	
	\begin{figure}[!ht]
		\centering
		\includegraphics[width=1\textwidth]{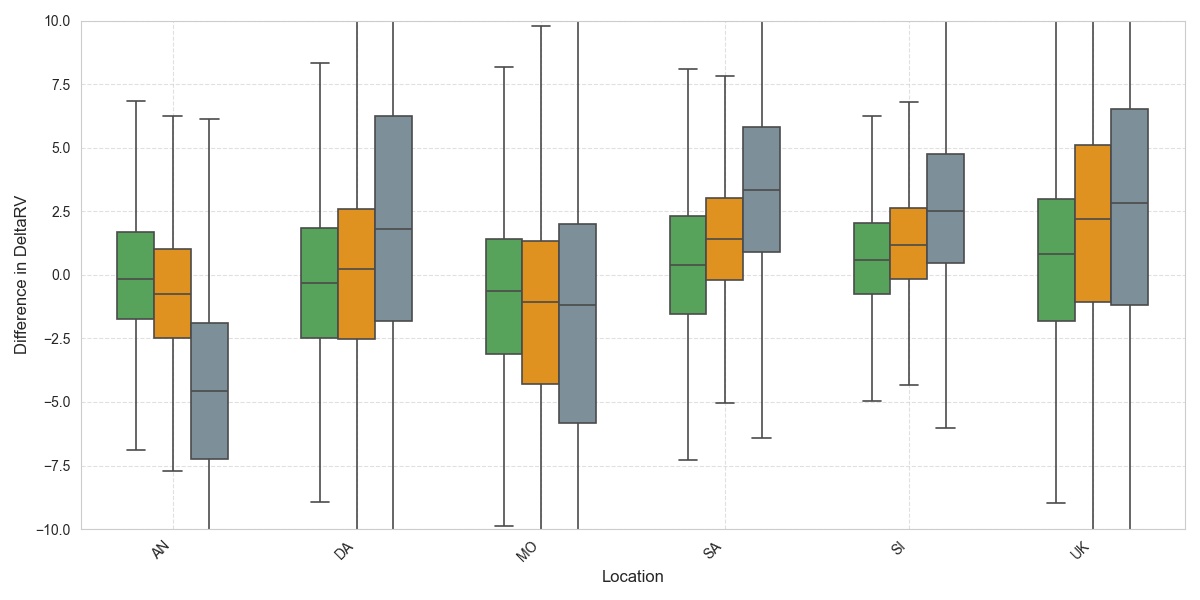}
		\caption{Summary of inferences for the difference $\Delta \Delta Q_j$, $j=1,2,3$ (see Equation~12) between $\Delta Q$ values of regional annual maxima and minima. AIC3 was used for model selection, and posterior distributions aggregated over climate ensemble and GCM. For other details, see Figure~8. For comparison with Figure~12.} 
		\label{Fgr-MxmMnmDff-BW-LctScn-DIC}
	\end{figure}
	
	%%%%%%%%%%%%%%%%%%%%%%%%%%%%%%%%%%%%%%%%%%%%%%%%%%%%%%%%%%%%%%%%%%
	\clearpage
	\FloatBarrier
	\section{Locations of regional annual maxima and minima in time} \label{SM:LctMxmMnm}
	%%%%%%%%%%%%%%%%%%%%%%%%%%%%%%%%%%%%%%%%%%%%%%%%%%%%%%%%%%%%%%%%%%
	%
	\begin{figure}[!ht]
		\centering
		\includegraphics[width=1\textwidth]{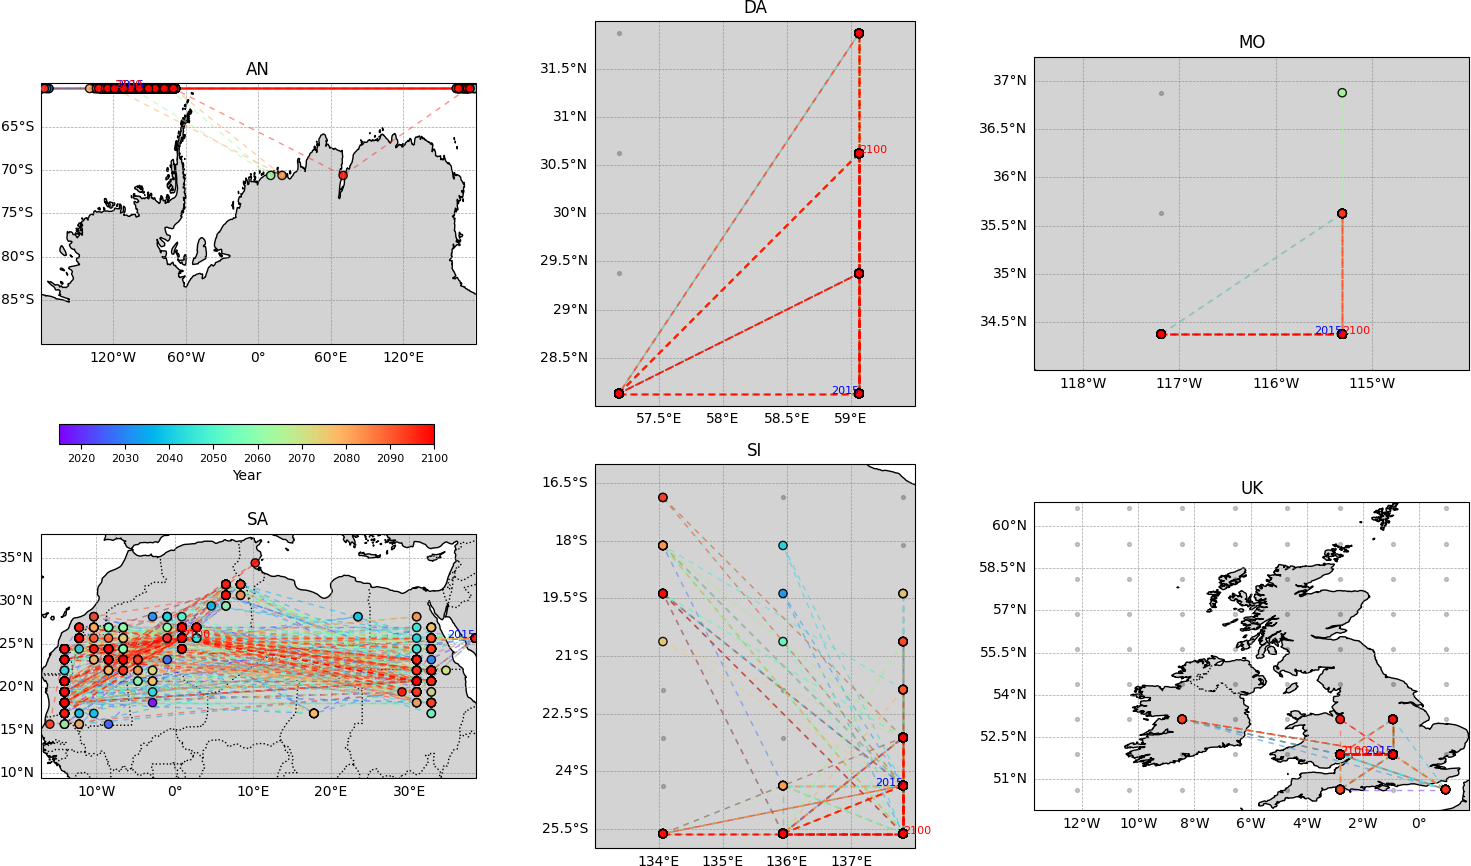}
		\caption{Locations of regional annual maxima (coloured discs) per region (panels) over time for the period (2015,2100) from the \UK GCM. Lines connect discs corresponding to adjacent years; disc and line colours indicate the year; grey dots indicate GCM grid locations for \DDA (DA), \DMO (MO), \DSI (SI) and \DUK (UK), suppressed for \DAN (AN) and \DSA (SA).} 
		\label{Fgr-Mxm-SptDst-UK}
	\end{figure}
	
	In this work we consider annual maxima and minima of \TA over different spatial domains. It is interesting to also consider whether there are spatial trends in the locations of regional maxima and minima in time for each region. Figure~\ref{Fgr-Mxm-SptDst-UK} shows the evolution of the location of regional annual maximum in time for the \UK GCM, with the ``time trajectory'' reverse-rainbow coloured from blue to red. For example, for the \DSA region, annual maxima tend to cluster in the dune seas south of the Atlas Mountains ($\approx$ ($10^\circ$W,$10^\circ$E)) and to the west of the Red Sea Hills ($\approx 30^\circ$E). For the \DAN, regional annual maxima generally occur at the northernmost grid locations within the bounding box. Corresponding plots for regional annual minima are given in Figure~SM71, and show obvious differences. For example, for the \DAN, minima tend of occur around Dome Argus ($\approx 75^\circ$E). For the \DSA, annual minima tend to occur in two clusters, each at $\approx 32^\circ$N, in the Atlas Mountains ($\approx 0^\circ$) and the Nafud desert, the Syrian Desert Highlands and the Southeastern Taurus Mountains ($\approx 40^\circ$E). Differences between the spatial locations of regional annual maxima and minima are clear for the \DDA, \DMO, \DSI and \DUK regions. For comparison, Figures~SM72-SM73 present analogous results for the \EC GCM, showing similar gross features. The presence of systematic spatial trends in the locations of extremes suggests, at least in principle, an opportunity for more sophisticated spatial modelling. However, there are no obvious trends in time in the locations of regional extrema.
	
	\begin{figure}[!ht]
		\centering
		\includegraphics[width=1\textwidth]{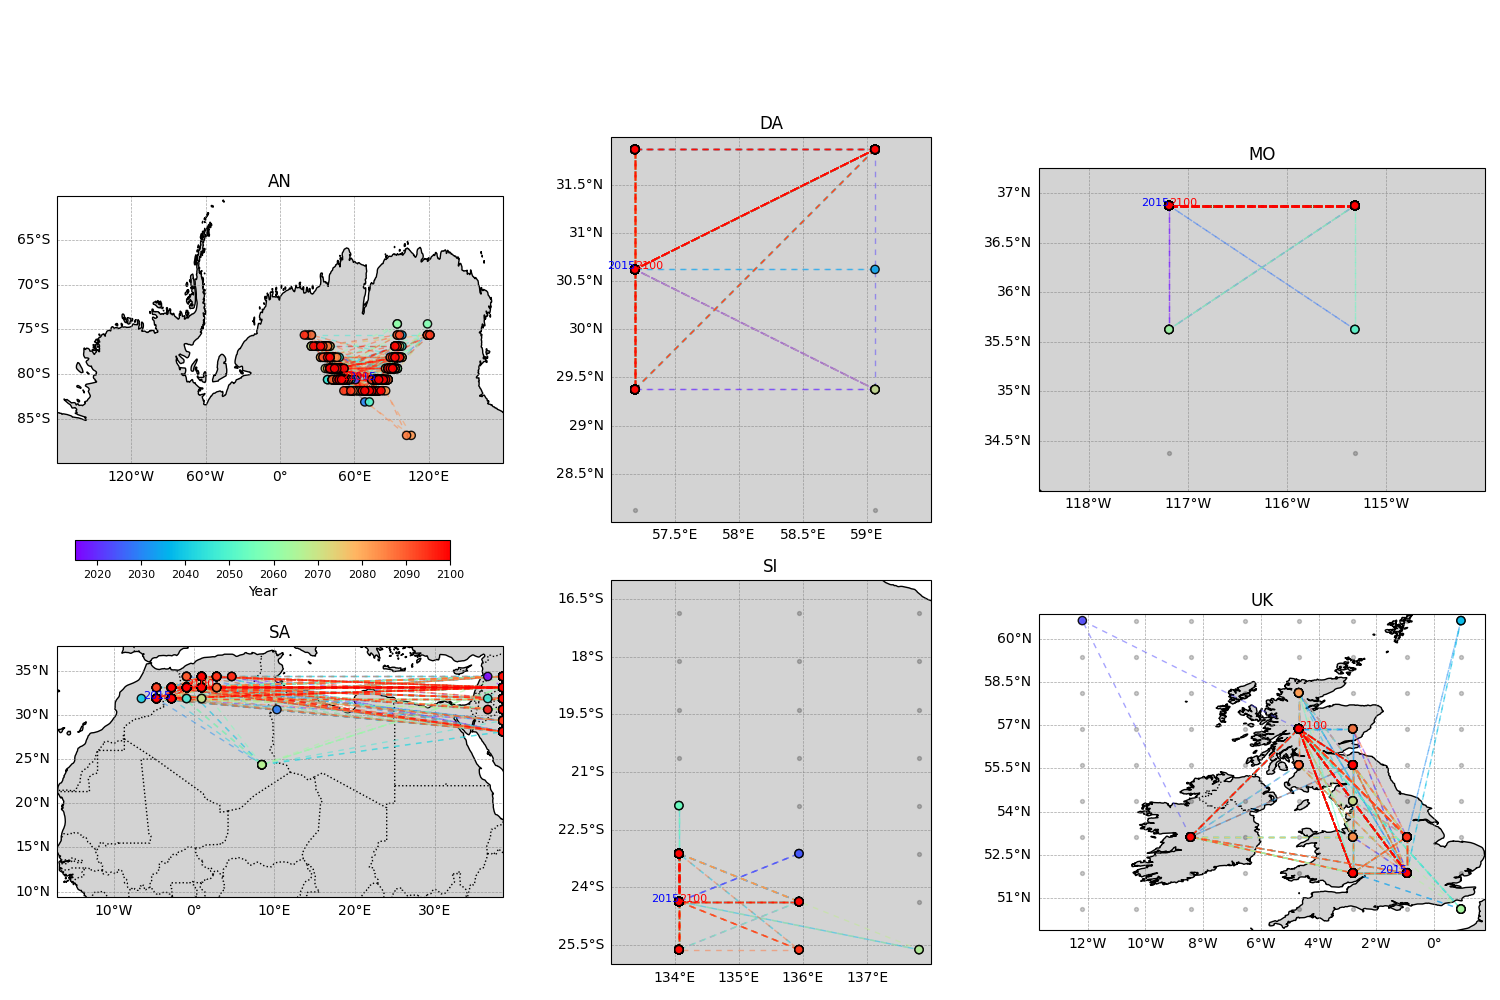}
		\caption{Locations of regional annual minima (coloured discs) per region (panels) over time for the period (2015,2100) from the \UK GCM. Lines connect discs corresponding to adjacent years; disc and line colours indicate the year; grey dots indicate GCM grid locations for \DDA (DA), \DMO (MO), \DSI (SI) and \DUK (UK), suppressed for \DAN (AN) and \DSA (SA).} 
		\label{Fgr-Mnm-SptDst-UK}
	\end{figure}
	
	\begin{figure}[!ht]
		\centering
		\includegraphics[width=1\textwidth]{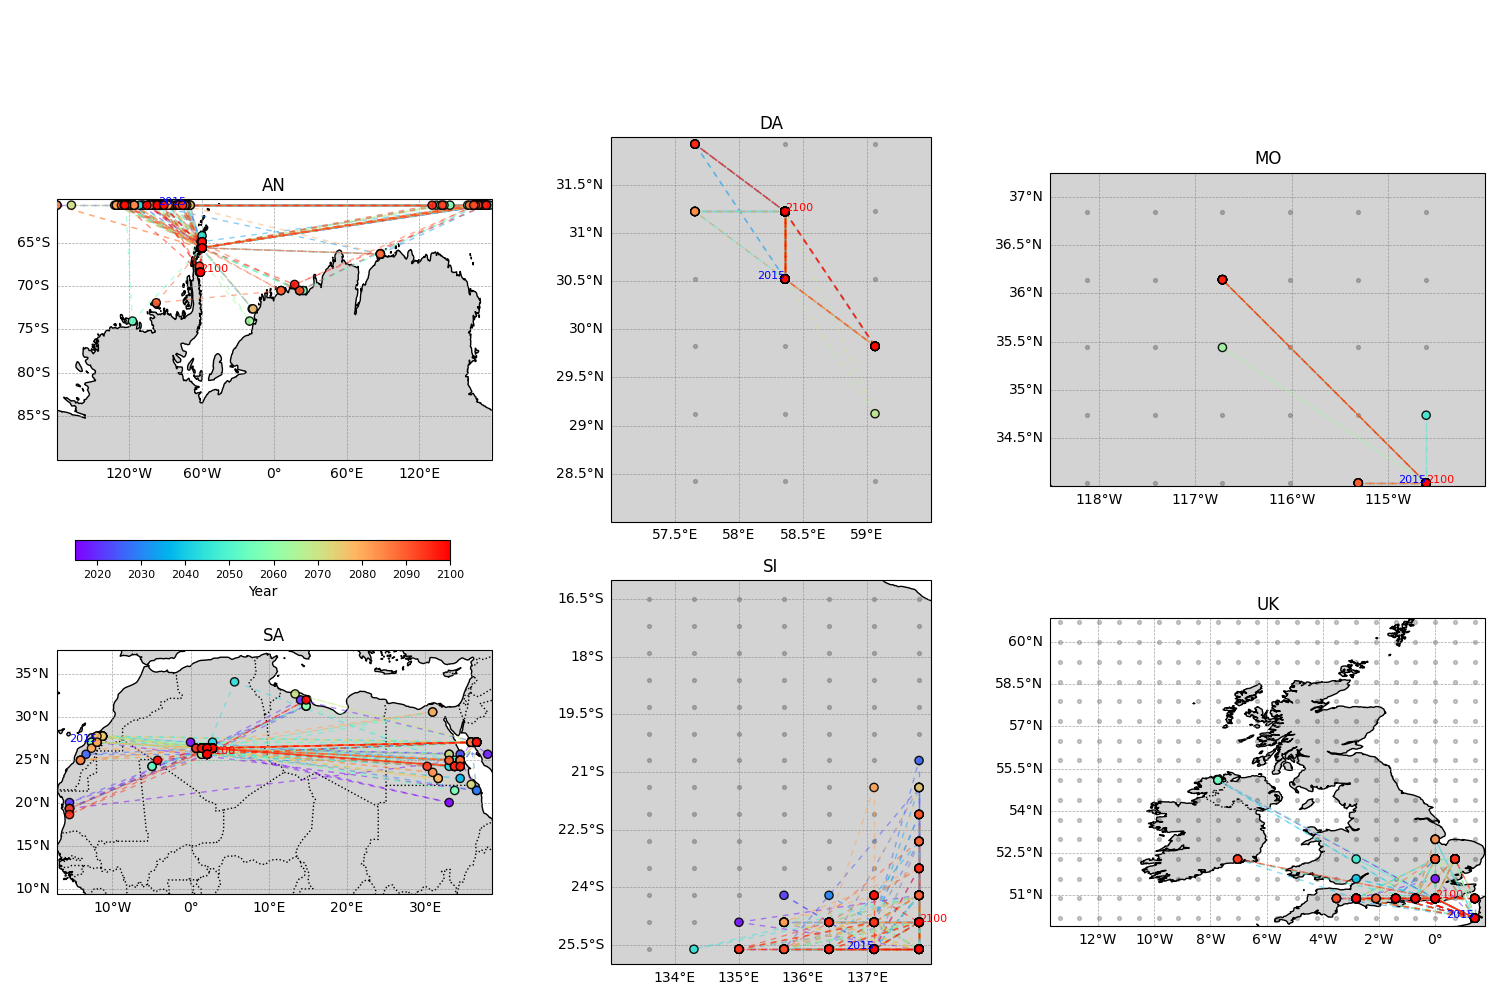}
		\caption{Locations of regional annual maxima (coloured discs) per region (panels) over time for the period (2015,2100) from the \EC GCM. For other details, see Figure~\ref{Fgr-Mxm-SptDst-UK}.} 
		\label{Fgr-Mxm-SptDst-EC}
	\end{figure}
	
	\begin{figure}[!ht]
		\centering
		\includegraphics[width=1\textwidth]{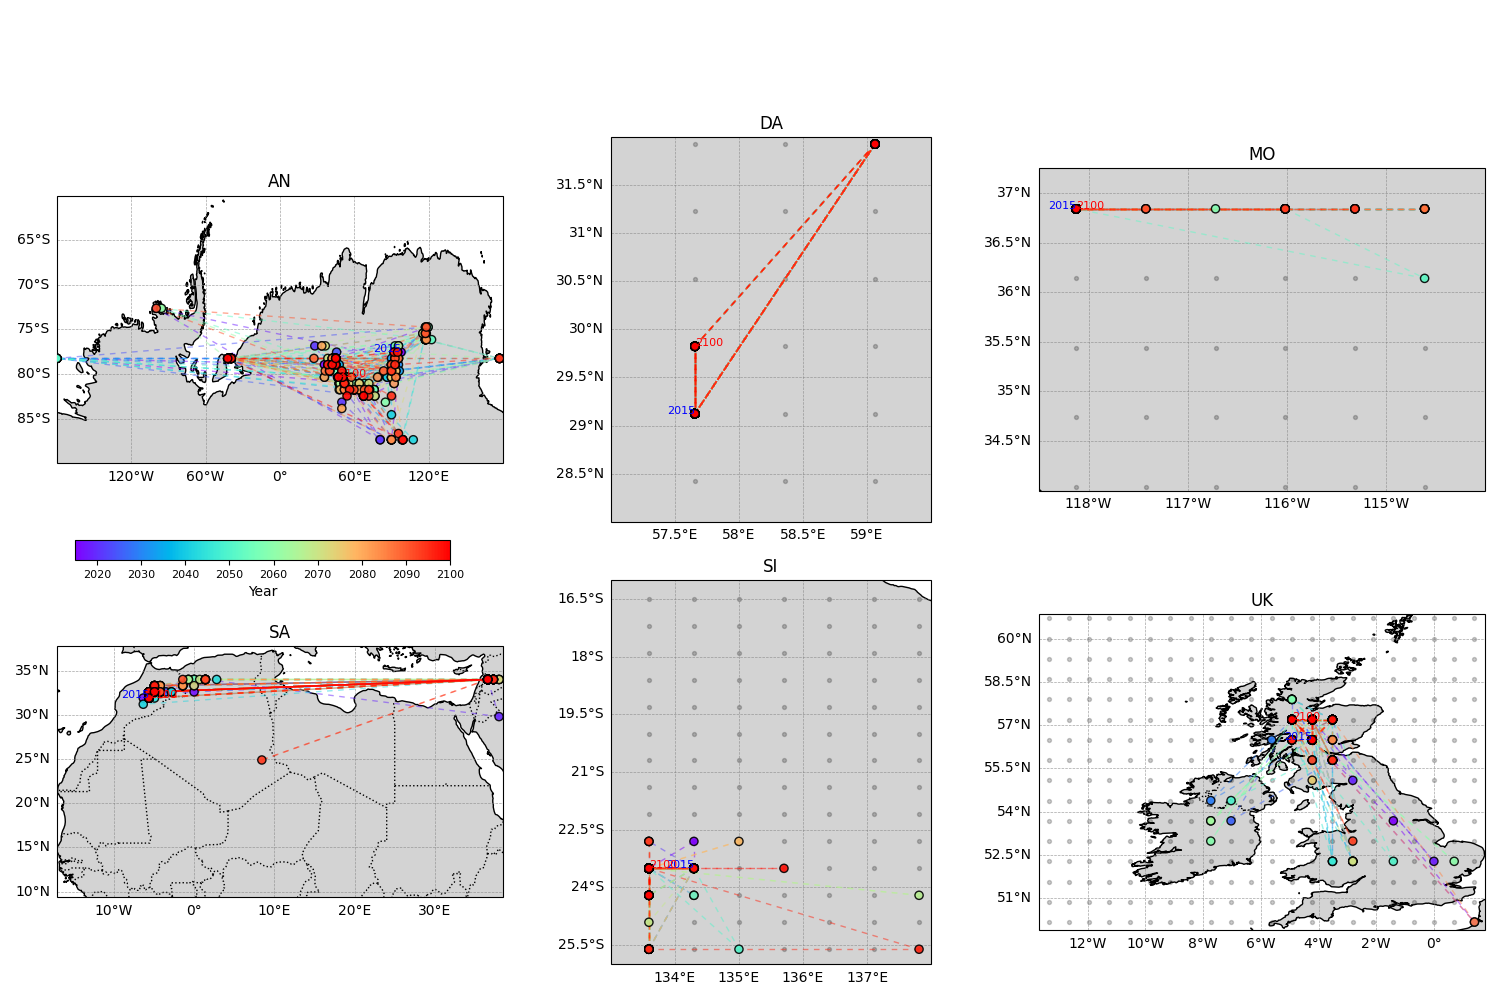}
		\caption{Locations of regional annual minima (coloured discs) per region (panels) over time for the period (2015,2100) from the \EC GCM. For other details, see Figure~\ref{Fgr-Mxm-SptDst-UK}.} 
		\label{Fgr-Mnm-SptDst-EC}
	\end{figure}
	
	%%%%%%%%%%%%%%%%%%%%%%%%%%%%%%%%%%%%%%%%%%%%%%%%%%%%%%%%%%%%%%%%%%
	\clearpage
	\FloatBarrier
	\section{Distribution of complexity of fitted models} \label{SM:DstMdlCmp}
	%%%%%%%%%%%%%%%%%%%%%%%%%%%%%%%%%%%%%%%%%%%%%%%%%%%%%%%%%%%%%%%%%%
	
	\begin{figure}[!ht]
		\centering
		\begin{subfigure}[b]{0.5\textwidth}
			\centering
			\caption*{Regional annual maxima}
			\includegraphics[width=1\textwidth]{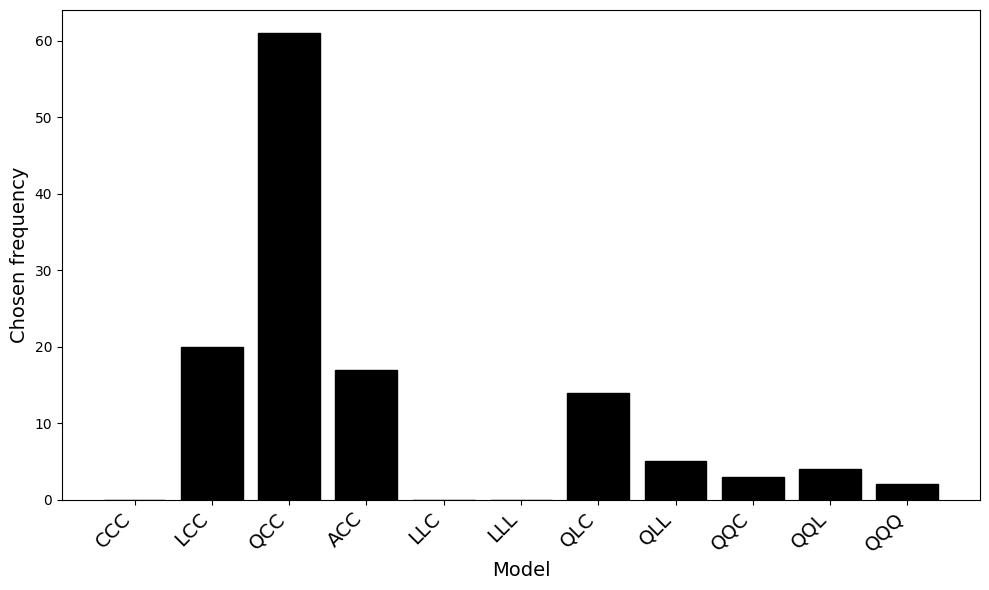}
		\end{subfigure}%
		\begin{subfigure}[b]{0.5\textwidth}
			\centering
			\caption*{Regional annual minima}
			\includegraphics[width=1\textwidth]{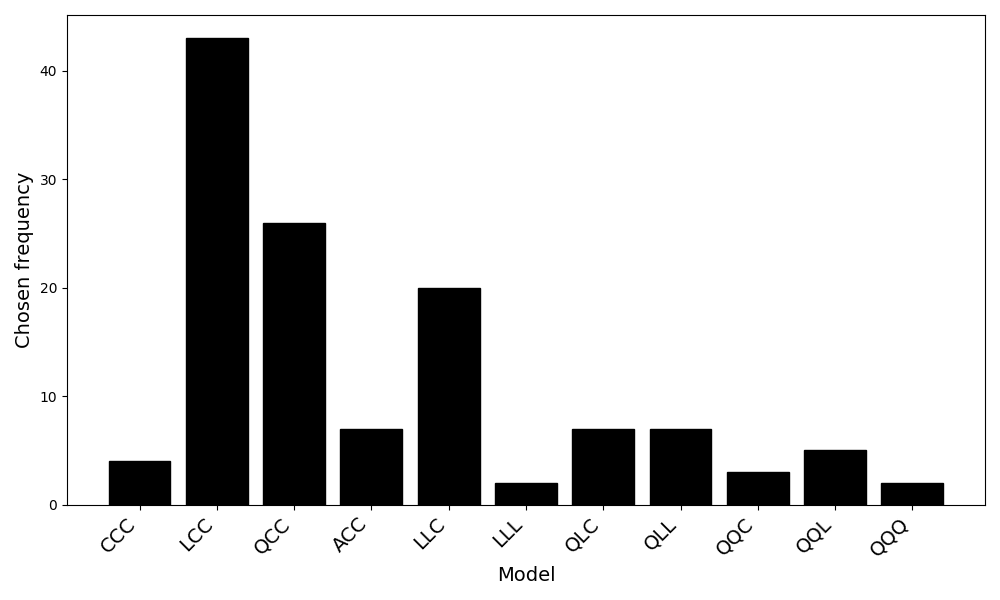}
		\end{subfigure}%
		\caption{Complexities of optimal fitted models for regional annual maxima (left) and minima (right) using AIC3 for model selection.} 
		\label{Fgr-Hst-MdlOrd-DIC}
	\end{figure}
	
	%%%%%%%%%%%%%%%%%%%%%%%%%%%%%%%%%%%%%%%%%%%%%%%%%%%%%%%%%%%%%%%%%%
	\clearpage
	\FloatBarrier
	\section{Bayesian model averaging} \label{SM:BMA}
	%%%%%%%%%%%%%%%%%%%%%%%%%%%%%%%%%%%%%%%%%%%%%%%%%%%%%%%%%%%%%%%%%%
	
	This section should be read in conjunction with Section~6.4 of the main text. Consider using sample $x=\{x_1, x_2, ..., x_P\}$ of annual maxima to estimate $n_M$ different models $M_1$, $M_2$, ..., $M_{n_M}$, with which to make a prediction of some future $q$. In the context of the current work, the $n_M=11$ models correspond to the different models CCC, LCC, ..., QQQ, and $q$ to the vector of values of $\Delta Q$ for the difference in 100-year return value between 2025 and 2125, for three climate scenarios \SL, \SM and \SH. Instead of selecting a single ``best'' model from the set of $n_M$ models, we can use a weighted average of all the models for prediction. Specifically, the Bayesian model average for the density $f(q|x)$ of $q$ given sample $x$ takes the form
	\begin{eqnarray} \label{Eqt:QGY}
		f(q|x)=\sum_{m=1}^{n_M} f(q|M_m, x) f(M_m|x)
	\end{eqnarray} 
	where $f(q|M_m, x)$ is the posterior predictive density of $q$ under model $M_m$, $m=1,2,$ ..., $n_M$, and $f(M_m|x)$ is the posterior probability of model $M_m$ given $x$. We can estimate $f(q|M_m, x)$ relatively straightforwardly using Bayesian inference, e.g., using MCMC as in the current work, since 
	\begin{eqnarray}  \label{Eqt:QGMkY}
		f(q|M_m, x)=\int_{\theta_m} f(q|\theta_m, M_m) f(\theta_m|M_m, x) d\theta
	\end{eqnarray} 
	where $f(\theta_m|M_m, x)$ is the posterior density of parameters $\theta_m$ of model $M_m$ from the MCMC, and $f(q|\theta_m, M_m)$ is the known density of $q$ given  $M_m$ and its parameters $\theta_m$. We can also attempt to estimate the posterior probability of model $M_m$ using the expression
	\begin{eqnarray}  \label{Eqt:MkGY}
		f(M_m|x)=\frac{f(x|M_m) f(M_m)}{\sum_{m'=1}^{n_M} f(x|M_{m'}) f(M_{m'})}
	\end{eqnarray} 
	where $f(x|M_m)$ is the marginal probability of $x$ under model $M_m$, given by
	\begin{eqnarray} \label{Eqt:MrgYGMk}
		f(x|M_m) = \int_{\theta_m} f(x|\theta_m, M_m) f(\theta_m|M_m) d\theta
	\end{eqnarray} 
	where $f(x|\theta_m, M_m)$ is the known density of $x$ given model $M_m$ with parameters $\theta_m$. The remaining densities $f(M_m)$ in Equation~\ref{Eqt:MkGY} and $f(\theta_m|M_m)$ in Equation~\ref{Eqt:MrgYGMk} are prior specifications of the models $M_m$, $m=1,2,$ ..., $n_M$ and their parameters $\theta_m$. In principle, once the priors are specified we can therefore use Equations~\ref{Eqt:QGY}~-~\ref{Eqt:MrgYGMk} to estimate the model average density for $q$.
	
	In practice however, specifying $f(M_m)$ and $f(\theta_m|M_m)$, $m=1,2,$ ..., $n_M$ is problematic. Practitioners often revert to trying different possible choices of prior, and confirming whether plausible estimates for $f(q|x)$ result. Model stacking provides a data-driven alternative to prior specification. The stacked model average density $f_S(q|x)$ is given by
	\begin{eqnarray} \label{Eqt:SQGY}
		f_S(q|x)=\sum_{m=1}^{n_M} w_m f(q|M_m, x)
	\end{eqnarray} 
	where weight vector $w=(w_1, w_2, ..., w_{n_M})$ is found by a cross-validation strategy
	\begin{eqnarray} \label{Eqt:SW}
		w=\argmax{w'} \sum_{i=1}^P \log\left(\sum_{m=1}^{n_M} w'_m f(x_i|M_m, x_{-i})\right)
	\end{eqnarray} 
	where $f(x_i|M_m, x_{-i})$ is the posterior predictive density of observation $x_i$, $i=1,2,$ ..., $n$, under model $M_m$ estimated using all observations in $x$ except for $x_i$. $f(x_i|M_m, x_{-i})$ is evaluated using
	\begin{eqnarray} \label{Eqt:MrgYGMkCV}
		f(x_i|M_m,x_{-i}) = \int_{\theta_m} f(x_i|\theta_m, M_m) f(\theta_m|M_m,x_{-i}) d\theta
	\end{eqnarray} 
	where, as before, $f(x_i|\theta_m, M_m)$ is a known density, and $f(\theta_m|M_m,x_{-i})$ is the posterior density of parameters $\theta_m$ of model $M_m$ estimated using sample $x_{-i}$, which can be sampled using MCMC. Comparison of Equations~\ref{Eqt:QGY} and \ref{Eqt:SQGY} suggests that the stacking weight vector $w$ acts as an estimate of the set of the posterior probabilities $f(M_m|x)$, $m=1,2,$ ..., $n_M$. 
	
	To then evaluate the RMSE for BMA in Section~6.4, we use the expression
	\begin{eqnarray}
		\text{RMSE} = \left(\frac{1}{3 n_R n_S} \sum_{j=1}^3 \sum_{k=1}^{n_R} \sum_{s=1}^{n_S} \left(\Delta Q_j^* - \sum_{m=1}^{n_M} (w_m|D_k) \left(\Delta Q_{j(s)}|M_m, D_k\right) \right)^2 \right)^{1/2}.
		\label{Eqt:RMSE-BMA}
	\end{eqnarray} 
	where $\Delta Q_j^*$ is the true value, and $\Delta Q_{j(s)}|M_m, D_k$ is posterior estimate of $\Delta Q_j$, $j=1,2,3$ corresponding to iteration $s$, $s=1,2,...,n_S$ from the MCMC chain for data realisation $D_k$, $k=1,2,...,n_R$ and model $M_m$, $m=1,2,...,n_M$, and $w_m|D_k$ is the BMA weight of model $M_m$ for data realisation $D_k$.
	
	Note that many different metrics (or ``scoring rules'') are available, as alternatives to RMSE, to evaluate the performance of our models for $\Delta Q$. We chose RMSE for its simplicity; an attractive option might be the Jensen-Shannon (JS) divergence. Clearly, the choice of preferred model selection criterion in the simulation study of S4 of the main text  (namely BIC3 using RMSE) might be different were we to use JS divergence as our metric.
	
	An issue with applications of leave-out methods to environmental extreme value modelling is that the support of an estimated marginal model $f(x|M_m)$ may be bounded above if the posterior density of the shape parameter is zero for non-negative values. As a result, it is possible in particular that the density $f(x|M_m, x_{-i})$ of withheld observation $x$ under model $M_m$ estimated using sample $x_{-i}$ is zero; that is, that the value $x$ lies beyond the upper end point of the estimated GEV distribution. To mitigate this issue, we impose a constraint on the Bayesian inference using MCMC, for each geographic region considered, that temperatures up to 20\% higher than the largest observed temperature (over all combinations of GCM, scenario and ensemble member) must have non-zero density. Formally, we insist that 
	\begin{eqnarray}
		\mu-\frac{\sigma}{\xi}>x_{\min}^*+1.2 \times (x_{\max}^*-x_{\min}^*)
	\end{eqnarray}
	for each geographic region, where $x_{\min}^*$ and $x_{\max}^*$ are the minimum and maximum values observed anywhere over the region, over all combinations of GCM, scenario and ensemble member.
	
	%%%%%%%%%%%%%%%%%%%%%%%%%%%%%%%%%%%%%%%%%%%%%%%%%%%%%%%%%%%%
	\ifNms
		\bibliographystyle{plainnat}
	\else
		\bibliographystyle{unsrtnat}
	\fi
	
	\bibliography{C:/Philip/Git/Cod/LaTeX/phil}
	%%%%%%%%%%%%%%%%%%%%%%%%%%%%%%%%%%%%%%%%%%%%%%%%%%%%%%%%%%%%
	
\end{document}
